# Supplementary material for: First-Order Primal-Dual Repairs for Scalable Branch and Bound
Source: arXiv:2610.26509 source file (2026-10-19)
Supplement: Supplementary file 1 [file 07_Appendix.tex]

\appendix
\papertitle{First-Order Primal-Dual Repairs for Scalable Branch and Bound:\\
Supplementary Materials}


\makeatletter
\newif\ifappcontentsvisible
\newcommand{\startappcontents}{\appcontentsvisibletrue}
\addtocontents{toc}{\protect\startappcontents}
\makeatother
\renewcommand{\contentsname}{Table of Contents}
\setcounter{tocdepth}{2}
\begingroup
\makeatletter
\let\originalcontentsline\contentsline
\renewcommand{\contentsline}[4]{%
  \ifappcontentsvisible
    \originalcontentsline{#1}{#2}{#3}{#4}%
  \fi
}
\makeatother
\tableofcontents
\endgroup
\clearpage

\input{sections/Appendix/B_primal_on_Conda_Vu}
\input{sections/Appendix/A_node_relaxation_and_feasible_dual}
\input{sections/Appendix/C_accurqacy_and_convergence_db}

\input{sections/Appendix/D_Quadratic_loss_conj_eval}

\input{sections/Appendix/E_primal_repair}

\input{sections/Appendix/F_anchor}

\input{sections/Appendix/G_problems_and_data}

\input{sections/Appendix/H_experiments}
