# Supplementary material for: First-Order Primal-Dual Repairs for Scalable Branch and Bound
Source: arXiv:2610.26509 source file (2026-10-19)
Supplement: Supplementary file 2 [file A_node_relaxation_and_feasible_dual.tex]

\section{Node Relaxation and Fenchel Dual}
\label{app:dual-bounds}

With the splitting method established in Appendix~\ref{sec:base-algorithm}, we derive the Fenchel dual of the node relaxation and prove the validity of the two lower-bound constructions introduced in Section~\ref{sec:methodology}. The derivation identifies the equality that couples the dual variables and explains why finite conjugate values alone do not guarantee a valid bound. We then show how to recover a lower bound by correcting one dual variable or accounting explicitly for the equality violation.
Our dual certificates build on~\citep{dunner2016primal,neumaier2004safe}; our contribution combines them with primal repair and residual-rate analysis in FOM-based BnB for convex MINLPs with tractable constraint-set projections and support functions.

\subsection{Constraint Representation and Fenchel Dual}
\label{app:fenchel}

Fix a node $\calN$ whose relaxation has a feasible point with finite objective value. Let $\bbeta\in\mathbb R^p$ denote the relaxed decision vector, $\bA\in\mathbb R^{n\times p}$ the loss matrix, and $\calB_{\calN}$ the node box. We assume that $f$, $g$, and the constraint functions $h_i$, $i\in[m]$, are proper, closed, and convex, with $f$ smooth and $\calB_{\calN}$ a nonempty closed convex box, possibly unbounded. We use the splitting in Section~\ref{subsec:convex-relaxation} and the main-text composite formulation: $g$ is the original nonsmooth objective term, and the node box is the zeroth constraint block,
\[
\calC_0:=\calB_{\calN},
\qquad
\calC_i:=\{\bbeta\in\mathbb R^p:h_i(\bbeta)\leq0\},
\quad i\in[m].
\]
We require tractable projections onto $\calC_i$ and evaluations of $\sigma_{\calC_i}$ for certificates; tractable $\operatorname{prox}_{h_i}$ alone does not suffice.
Here, $\delta_{\calC}$ equals zero on $\calC$ and $+\infty$ elsewhere. We represent the node box and the additional inequalities through
\[
\bK:=\begin{bmatrix}\bI_p\\\vdots\\\bI_p\end{bmatrix}\in\mathbb R^{(m+1)p\times p},
\qquad
h(\bq_0,\ldots,\bq_m):=\sum_{i=0}^m\delta_{\calC_i}(\bq_i).
\]
Thus, $\bK$ stacks $m+1$ copies of the identity, and $h$ contains all constraint indicators, including the node box. We do not absorb $\delta_{\calB_{\calN}}$ into $g$. The node relaxation becomes
\begin{align}
p_{\calN}^\star&=\inf_{\bbeta\in\mathbb R^p}p_{\calN}(\bbeta),
\label{eq:app-node}\\
p_{\calN}(\bbeta)&:=f(\bA\bbeta)+g(\bbeta)+h(\bK\bbeta).
\label{eq:app-split}
\end{align}
We write $\operatorname{dom}p_{\calN}:=\{\bbeta:p_{\calN}(\bbeta)<+\infty\}$ for the points that satisfy the node constraints and have finite objective value. In particular, $h(\bK\bbeta)=0$ for every $\bbeta\in\operatorname{dom}p_{\calN}$.

For a proper function $\psi$, its Fenchel conjugate is
\[
\psi^*(\bv):=\sup_{\bx}\{\langle\bv,\bx\rangle-\psi(\bx)\}.
\]
Applying this definition to an indicator gives the support function:
\begin{equation}
\delta_{\calC}^*(\bv)=\sigma_{\calC}(\bv):=\sup_{\bx\in\calC}\langle\bv,\bx\rangle.
\label{eq:app-support}
\end{equation}

To derive the dual, we separate the arguments of $f$, $g$, and $h$ by introducing copies $\by\in\mathbb R^n$, $\bv\in\mathbb R^p$, and $\bq\in\mathbb R^{(m+1)p}$, with
\[
\by=\bA\bbeta,
\qquad
\bv=\bbeta,
\qquad
\bq=\bK\bbeta.
\]
We associate these equalities with multipliers $\bzeta\in\mathbb R^n$, $\bu\in\mathbb R^p$, and $\bnu=(\bnu_0,\ldots,\bnu_m)\in\mathbb R^{(m+1)p}$, respectively. The Lagrangian of this lifted formulation is
\[
\begin{aligned}
&f(\by)+g(\bv)+h(\bq)\\
&\quad+\langle\bzeta,\bA\bbeta-\by\rangle+\langle\bu,\bbeta-\bv\rangle+\langle\bnu,\bK\bbeta-\bq\rangle.
\end{aligned}
\]
Minimizing over the copies $\by$, $\bv$, and $\bq$ gives
\[
d(\bzeta,\bu,\bnu)+\langle V(\bzeta,\bu,\bnu),\bbeta\rangle,
\]
where the block indices follow the composite formulation,
\begin{align*}
d(\bzeta,\bu,\bnu)&:=-f^*(\bzeta)-g^*(\bu)-h^*(\bnu),\\
h^*(\bnu)&=\sum_{i=0}^m\sigma_{\calC_i}(\bnu_i)=\sigma_{\calB_{\calN}}(\bnu_0)+\sum_{i=1}^m\sigma_{\calC_i}(\bnu_i),\\
V(\bzeta,\bu,\bnu)&:=\bA^\top\bzeta+\bu+\bK^\top\bnu.
\end{align*}
The node box acts on the zeroth copy $\bq_0$ through $\delta_{\calB_{\calN}}(\bq_0)$, so $\bbeta$ remains unrestricted in the Lagrangian minimization. In particular, the support term $\sigma_{\calB_{\calN}}(\bnu_0)$ must be included in every evaluation of $h^*$ under this splitting. Consequently,
\[
\inf_{\bbeta\in\mathbb R^p}\langle V(\bzeta,\bu,\bnu),\bbeta\rangle=
\begin{cases}
0, & V(\bzeta,\bu,\bnu)=\vzero,\\
-\infty, & V(\bzeta,\bu,\bnu)\neq\vzero.
\end{cases}
\]
Indeed, when the violation is nonzero, choosing $\bbeta=-tV(\bzeta,\bu,\bnu)$ and letting $t\to+\infty$ makes the inner product tend to $-\infty$. We therefore obtain the Fenchel dual
\begin{equation}
d^\star:=\sup_{\bzeta,\bu,\bnu}\{d(\bzeta,\bu,\bnu):V(\bzeta,\bu,\bnu)=\vzero\}\leq p_{\calN}^\star.
\label{eq:app-dual-canonical}
\end{equation}
The inequality follows from weak duality. A tuple with finite conjugate values and $V(\bzeta,\bu,\bnu)=\vzero$ therefore provides a finite lower bound. When the equality fails, evaluating $d$ alone does not in general provide a valid bound. The next two constructions address this violation without requiring the underlying iteration to converge.

\subsection{Dual Feasibility Repair}
\label{app:dual-repair}

The variable $\bu$ enters the dual equality through the identity, so we can enforce the equality by changing $\bu$ while keeping $\bzeta$ and $\bnu$ fixed. To obtain a finite lower bound, we must also ensure that $g^*$ remains finite at the corrected point.

\begin{proposition}[Absorbing repair]
\label{prop:app-absorbing}
Suppose that $f^*(\bzeta)$ and $h^*(\bnu)$ are finite and that $\operatorname{dom}g^*=\mathbb R^p$. Define
\begin{equation}
\widetilde{\bu}:=-\bA^\top\bzeta-\bK^\top\bnu.
\label{eq:app-u-repair}
\end{equation}
Then $(\bzeta,\widetilde{\bu},\bnu)$ satisfies the dual equality, has finite conjugate values, and gives the lower bound
\begin{equation}
\mathrm{LB}_{\mathrm{repair}}(\bzeta,\bu,\bnu):=d(\bzeta,\widetilde{\bu},\bnu)\leq d^\star\leq p_{\calN}^\star.
\label{eq:app-d-repair}
\end{equation}
\end{proposition}

\begin{proof}
For any candidate $\bu\in\mathbb R^p$, subtracting its equality violation gives
\[
\begin{aligned}
\bu-V(\bzeta,\bu,\bnu)
&=\bu-(\bA^\top\bzeta+\bu+\bK^\top\bnu)\\
&=-\bA^\top\bzeta-\bK^\top\bnu=\widetilde{\bu}.
\end{aligned}
\]
Substituting the corrected variable into the dual equality yields
\[
V(\bzeta,\widetilde{\bu},\bnu)=\bA^\top\bzeta+\widetilde{\bu}+\bK^\top\bnu=\vzero.
\]
The full-domain assumption ensures that $g^*(\widetilde{\bu})$ is finite. The other two conjugates are finite by hypothesis, so $d(\bzeta,\widetilde{\bu},\bnu)$ is a finite feasible dual value. Equation~\eqref{eq:app-dual-canonical} gives the claimed inequalities.
\end{proof}

The full-domain assumption guarantees finiteness for every correction; for an individual tuple, the proof only requires $g^*(\widetilde{\bu})<+\infty$. One sufficient condition for the full-domain assumption is that $g$ have bounded domain and a finite lower bound~\citep{dunner2016primal}. Specifically, if $\|\bbeta\|_2\leq R_g$ and $g(\bbeta)\geq\underline g$ on $\operatorname{dom}g$, for finite constants $R_g\geq0$ and $\underline g$, then
\[
\begin{aligned}
g^*(\bu)
&=\sup_{\bbeta\in\operatorname{dom}g}\{\langle\bu,\bbeta\rangle-g(\bbeta)\}\\
&\leq R_g\|\bu\|_2-\underline g<+\infty
\qquad\text{for every }\bu\in\mathbb R^p.
\end{aligned}
\]
These bounds must cover the full domain of $g$ in the full decision space, including any explicit selector variables. Boundedness of the node box alone does not establish this condition, because its indicator belongs to $h$, not to $g$. For example, $g\equiv0$ has $g^*=\delta_{\{\vzero\}}$, so a nonzero correction of $\bu$ yields only the trivial lower bound $-\infty$. A finite repaired bound therefore requires the stated conjugate-domain condition; when applicable, the residual correction below provides an alternative.

Because $\widetilde{\bu}$ depends only on $\bzeta$ and $\bnu$, we need not update $\bu$ independently to evaluate the repaired bound. Eliminating $\bu$ from the dual equality also gives the equivalent reduced dual
\[
d^\star=\sup_{\bzeta,\bnu}\{-f^*(\bzeta)-g^*(-\bA^\top\bzeta-\bK^\top\bnu)-h^*(\bnu)\},
\]
where we interpret the objective as $-\infty$ whenever a conjugate is infinite.

\subsection{Residual-Corrected Lower Bound}
\label{app:residual-bound}

Alternatively, we keep the candidate tuple unchanged and account for the equality violation in the bound itself. We do this by bounding its contribution over a known convex set containing $\operatorname{dom}p_{\calN}$. Unlike the absorbing repair, this construction does not require evaluating $g^*$ at a corrected argument.

\begin{proposition}[Residual correction]
\label{prop:app-residual}
Let $(\bzeta,\bu,\bnu)$ have finite conjugate values. Suppose that $\calD\subseteq\mathbb R^p$ is nonempty, closed, and convex, with $\operatorname{dom}p_{\calN}\subseteq\calD$ and $\sigma_{\calD}(-V(\bzeta,\bu,\bnu))<+\infty$. Then
\begin{equation}
\begin{aligned}
\mathrm{LB}_{\mathrm{violation}}(\bzeta,\bu,\bnu)
&:=d(\bzeta,\bu,\bnu)-\sigma_{\calD}(-V(\bzeta,\bu,\bnu))\\
&\leq p_{\calN}^\star
\end{aligned}
\label{eq:app-d-res}
\end{equation}
is a finite lower bound, including when $V(\bzeta,\bu,\bnu)\neq\vzero$.
\end{proposition}

\begin{proof}
Fix any $\bbeta\in\operatorname{dom}p_{\calN}$. Applying the Fenchel--Young inequality to each term and using $h(\bK\bbeta)=0$ gives
\begin{align*}
f(\bA\bbeta)&\geq\langle\bzeta,\bA\bbeta\rangle-f^*(\bzeta),\\
g(\bbeta)&\geq\langle\bu,\bbeta\rangle-g^*(\bu),\\
0&\geq\langle\bnu,\bK\bbeta\rangle-h^*(\bnu).
\end{align*}
Adding these inequalities yields
\[
p_{\calN}(\bbeta)\geq d(\bzeta,\bu,\bnu)+\langle V(\bzeta,\bu,\bnu),\bbeta\rangle.
\]
Taking the infimum over $\operatorname{dom}p_{\calN}$ and using $\operatorname{dom}p_{\calN}\subseteq\calD$, we obtain
\begin{align*}
p_{\calN}^\star
&\geq d(\bzeta,\bu,\bnu)+\inf_{\bbeta\in\operatorname{dom}p_{\calN}}\langle V(\bzeta,\bu,\bnu),\bbeta\rangle\\
&\geq d(\bzeta,\bu,\bnu)+\inf_{\bbeta\in\calD}\langle V(\bzeta,\bu,\bnu),\bbeta\rangle\\
&=d(\bzeta,\bu,\bnu)-\sigma_{\calD}(-V(\bzeta,\bu,\bnu))\\
&=\mathrm{LB}_{\mathrm{violation}}(\bzeta,\bu,\bnu).
\end{align*}
Both $d(\bzeta,\bu,\bnu)$ and the support-function correction are finite by assumption.
\end{proof}

Known coordinate bounds give a simple choice of $\calD$~\citep{neumaier2004safe,applegate2021practical}. Suppose that $L_j\leq\beta_j\leq U_j$ for every $\bbeta\in\operatorname{dom}p_{\calN}$ and $j\in[p]$, with finite $L_j$ and $U_j$. Taking $\calD=\prod_{j=1}^p[L_j,U_j]$, we can evaluate the correction coordinatewise:
\[
\sigma_{\calD}(-V(\bzeta,\bu,\bnu))=\sum_{j=1}^p\max\{-L_jV_j,-U_jV_j\},
\qquad V_j:=[V(\bzeta,\bu,\bnu)]_j.
\]
When $V(\bzeta,\bu,\bnu)=\vzero$, the correction vanishes and $\mathrm{LB}_{\mathrm{violation}}(\bzeta,\bu,\bnu)=d(\bzeta,\bu,\bnu)$.

Both constructions provide valid lower bounds under their respective finiteness conditions, independently of convergence of the iteration that generates the candidate tuple. For the iteration described in Appendix~\ref{sec:base-algorithm}, Appendix~\ref{app:methodology-proofs} next proves the residual-to-error estimates in Theorem~\ref{theorem:convergence_rate}.
