# Supplementary material for: First-Order Primal-Dual Repairs for Scalable Branch and Bound
Source: arXiv:2610.26509 source file (2026-10-19)
Supplement: Supplementary file 3 [file B_primal_on_Conda_Vu.tex]

\section{Primer on the Primal--Dual Splitting Method and the Condat--V\~u Algorithm}
\label{sec:base-algorithm}

We derive the Condat-V\~u iteration used in the main text and establish its convergence through preconditioned forward-backward splitting~\citep[Section~3.3]{ryuyin2022largescale}. We start from the node formulation in Problem~\eqref{problem:relaxation_in_composite_form}: $g$ is the original nonsmooth objective term, $h$ collects the node-box indicator as block $0$ together with the $m$ additional constraint indicators, and $\bK\in\mathbb R^{(m+1)p\times p}$ stacks $m+1$ copies of the identity. The node $\calN$ remains fixed throughout this section. Appendix~\ref{app:dual-bounds} then derives the Fenchel dual and the two safe lower bounds, whose residual-based error estimates are proved in Appendix~\ref{app:methodology-proofs}.

We assume that $f:\mathbb R^n\to\mathbb R$ is convex and differentiable, with an $L_f$-Lipschitz gradient for some $L_f>0$:
\begin{equation}
\norm{\nabla f(\by)-\nabla f(\widehat{\by})}_2\leq L_f\norm{\by-\widehat{\by}}_2
\qquad\text{for all }\by,\widehat{\by}\in\mathbb R^n.
\label{eq:base-loss-smoothness}
\end{equation}
For a differentiable convex function on $\mathbb R^n$, this is equivalent to the quadratic upper bound
\begin{equation}
f(\by)\leq f(\widehat{\by})+\ip{\nabla f(\widehat{\by})}{\by-\widehat{\by}}+\frac{L_f}{2}\norm{\by-\widehat{\by}}_2^2.
\label{eq:base-loss-descent}
\end{equation}
We also assume that $g$ and $h$ are proper, closed, and convex, that their proximal operators can be evaluated efficiently, and that the saddle-point problem below has a solution. All vector norms without a metric subscript are Euclidean, and $\norm{\bA}_2$ and $\norm{\bK}_2$ denote spectral norms.

\subsection{Saddle-point Formulation and Preconditioned Forward--Backward Splitting}

The node relaxation admits the saddle-point formulation
\begin{equation}
\inf_{\bbeta}\sup_{\bnu}\calL(\bbeta,\bnu),
\qquad
\calL(\bbeta,\bnu):=f(\bA\bbeta)+g(\bbeta)+\ip{\bnu}{\bK\bbeta}-h^*(\bnu).
\label{problem:saddle-point-formulation}
\end{equation}
Let $\bw:=(\bbeta,\bnu)\in\mathbb R^p\times\mathbb R^{(m+1)p}$. The saddle-point optimality conditions are
\begin{equation}
\vzero\in
\begin{bmatrix}
\bA^\top\nabla f(\bA\bbeta)+\partial g(\bbeta)+\bK^\top\bnu\\
\partial h^*(\bnu)-\bK\bbeta
\end{bmatrix}
=(\calA+\calS)(\bw),
\label{eq:base-saddle-operator}
\end{equation}
where
\begin{equation}
\calA(\bw):=
\begin{bmatrix}
\partial g(\bbeta)\\
\partial h^*(\bnu)
\end{bmatrix}
+
\begin{bmatrix}
0&\bK^\top\\
-\bK&0
\end{bmatrix}\bw,
\qquad
\calS(\bw):=
\begin{bmatrix}
\bA^\top\nabla f(\bA\bbeta)\\
\vzero
\end{bmatrix}.
\label{eq:base-operators}
\end{equation}
The set-valued operator $\calA$ contains the subdifferentials of the convex functions $g$ and $h^*$ together with the skew-symmetric coupling. The single-valued operator $\calS$ contains the gradient of the composite loss $f\circ\bA$. Thus, a pair $\bw^\star=(\bbeta^\star,\bnu^\star)$ is a saddle point exactly when
\begin{equation}
\vzero\in(\calA+\calS)(\bw^\star).
\label{eq:base-zero-inclusion}
\end{equation}

A direct forward--backward construction gives the fixed-point characterization
\begin{equation}
\bw^\star=T_0\bw^\star,
\qquad
T_0:=(\calI+\calA)^{-1}\circ(\calI-\calS),
\label{eq:base-unpreconditioned-map}
\end{equation}
where $\calI$ is the identity operator. The forward step evaluates $\calS$ at the current point, while the resolvent $(\calI+\calA)^{-1}$ performs the implicit backward step. If $\calA$ contained only the two subdifferentials, its resolvent would separate into two proximal evaluations. The skew-symmetric term instead couples the new primal and dual variables. Equation~\eqref{eq:base-unpreconditioned-map} characterizes the saddle points, but does not by itself guarantee convergence of the unit-step iteration.

We choose the symmetric preconditioning matrix
\begin{equation}
\bM:=
\begin{bmatrix}
\sigma^{-1}\bI_p&-\bK^\top\\
-\bK&\tau^{-1}\bI_{(m+1)p}
\end{bmatrix},
\qquad \sigma>0,\quad\tau>0,
\label{eq:base-metric}
\end{equation}
with step sizes such that $\bM\succ0$. We give an explicit sufficient condition for convergence in Section~\ref{sec:base-cv-convergence}. Since $\bM$ is invertible, the optimality inclusion is equivalent to
\begin{equation}
\vzero\in(\bM^{-1}\calA+\bM^{-1}\calS)(\bw^\star).
\label{eq:base-preconditioned-inclusion}
\end{equation}
Applying forward--backward splitting in this metric gives
\begin{equation}
\bw^\star=T\bw^\star,
\qquad
T:=(\calI+\bM^{-1}\calA)^{-1}\circ(\calI-\bM^{-1}\calS).
\label{eq:base-cv-map}
\end{equation}
The preconditioner preserves the saddle points and, as we show next, makes the backward step separable into two sequential proximal evaluations.

\subsection{Condat--V\~u Algorithm}

Write $\bw^+:=T\bw$, where $\bw=(\bbeta,\bnu)$ and $\bw^+=(\bbeta^+,\bnu^+)$. The definition of the resolvent gives
\[
\bw-\bM^{-1}\calS(\bw)\in\bw^++\bM^{-1}\calA(\bw^+).
\]
Multiplying by $\bM$, we obtain
\begin{equation}
\bM\bw-\calS(\bw)\in\bM\bw^++\calA(\bw^+).
\label{eq:base-cv-step-inclusion}
\end{equation}
The upper-right block of $\bM$ cancels the corresponding block of the skew-symmetric coupling:
\begin{equation}
\underbrace{
\begin{bmatrix}
\sigma^{-1}\bI_p&-\bK^\top\\
-\bK&\tau^{-1}\bI_{(m+1)p}
\end{bmatrix}}_{\bM}
+
\begin{bmatrix}
0&\bK^\top\\
-\bK&0
\end{bmatrix}
=
\underbrace{
\begin{bmatrix}
\sigma^{-1}\bI_p&0\\
-2\bK&\tau^{-1}\bI_{(m+1)p}
\end{bmatrix}}_{\text{block lower triangular}}.
\label{eq:base-cv-triangular-matrix}
\end{equation}
Substituting into Equation~\eqref{eq:base-cv-step-inclusion} gives
\begin{equation}
\begin{bmatrix}
\sigma^{-1}\bbeta-\bK^\top\bnu-\bA^\top\nabla f(\bA\bbeta)\\
\tau^{-1}\bnu-\bK\bbeta
\end{bmatrix}
\in
\begin{bmatrix}
\sigma^{-1}\bI_p&0\\
-2\bK&\tau^{-1}\bI_{(m+1)p}
\end{bmatrix}
\begin{bmatrix}
\bbeta^+\\
\bnu^+
\end{bmatrix}
+
\begin{bmatrix}
\partial g(\bbeta^+)\\
\partial h^*(\bnu^+)
\end{bmatrix}.
\label{eq:base-cv-matrix-form}
\end{equation}
The first block involves only the new primal variable $\bbeta^+$. Once we compute it, the second block determines $\bnu^+$. Rearranging the two inclusions gives
\begin{align*}
\bbeta-\sigma\bigl(\bA^\top\nabla f(\bA\bbeta)+\bK^\top\bnu\bigr)
&\in\bbeta^++\sigma\partial g(\bbeta^+),\\
\bnu+\tau\bK(2\bbeta^+-\bbeta)
&\in\bnu^++\tau\partial h^*(\bnu^+).
\end{align*}
For a proper, closed, convex function $\psi$ and $\rho>0$, the proximal operator satisfies
\[
\prox_{\rho\psi}(\bv):=\arg\min_{\bx}\left\{\psi(\bx)+\frac{1}{2\rho}\norm{\bx-\bv}_2^2\right\}
=(\calI+\rho\partial\psi)^{-1}(\bv).
\]
We therefore recover the Condat--V\~u update from the main text:
\begin{equation}
\begin{aligned}
T\bw&=(\bbeta^+,\bnu^+),\qquad\text{where}\\
\bbeta^+&=\prox_{\sigma g}\!\left(\bbeta-\sigma\bigl(\bA^\top\nabla f(\bA\bbeta)+\bK^\top\bnu\bigr)\right),\\
\bnu^+&=\prox_{\tau h^*}\!\left(\bnu+\tau\bK(2\bbeta^+-\bbeta)\right).
\end{aligned}
\label{eq:base-cv-update}
\end{equation}
Here, $\sigma$ and $\tau$ are the primal and dual step sizes, respectively. When we have access to the proximal operator of $h$, Moreau's identity gives the required dual proximal operator~\citep{bauschke2017convex}:
\[
\prox_{\tau h^*}(\bv)=\bv-\tau\prox_{h/\tau}(\bv/\tau).
\]
The update uses gradient evaluations, matrix--vector products, and proximal maps; it does not require forming or inverting $\bM$. It also ensures $\bbeta^+\in\operatorname{dom}g$ and $\bnu^+\in\operatorname{dom}h^*$. Since the node box is represented in $h$, the primal proximal update alone does not ensure $\bbeta^+\in\calB_{\calN}$. The node-feasibility hypothesis used for the segment repair in Appendix~\ref{app:primal-repair} must therefore be checked separately. Repeated application gives the base iteration $\bw^{t+1}=T\bw^t$.

\subsection{Convergence of the Condat--V\~u Algorithm}
\label{sec:base-cv-convergence}

We prove convergence of the fixed-step iteration $\bw^{t+1}=T\bw^t$. Since $\bM\succ0$, it defines an inner product and norm on $\mathbb R^p\times\mathbb R^{(m+1)p}$:
\begin{equation}
\ip{\bw}{\widehat{\bw}}_{\bM}:=\bw^\top\bM\widehat{\bw},
\qquad
\norm{\bw}_{\bM}:=\sqrt{\ip{\bw}{\bw}_{\bM}}.
\label{eq:base-metric-norm}
\end{equation}
An operator $U$ is nonexpansive in this metric if
\[
\norm{U\bw-U\widehat{\bw}}_{\bM}\leq\norm{\bw-\widehat{\bw}}_{\bM}
\qquad\text{for all }\bw,\widehat{\bw}.
\]
It is $\alpha$-averaged, for $\alpha\in(0,1)$, if $U=(1-\alpha)\calI+\alpha\calR$ for some nonexpansive operator $\calR$. We establish this property for $T$ by analyzing its two factors:
\begin{equation}
T=T_1\circ T_2,
\qquad
T_1:=(\calI+\bM^{-1}\calA)^{-1},
\qquad
T_2:=\calI-\bM^{-1}\calS.
\label{eq:base-cv-factors}
\end{equation}
All averagedness and nonexpansiveness statements below use the same $\bM$-induced metric.

\paragraph{Step 1: the backward map $T_1$ is $1/2$-averaged.}

The product operator $(\bbeta,\bnu)\mapsto\partial g(\bbeta)\times\partial h^*(\bnu)$ is maximally monotone. The skew-symmetric coupling is linear, continuous, and monotone on the entire product space, so adding it preserves maximal monotonicity~\citep{bauschke2017convex}. Hence $\calA$ is maximally monotone. Multiplication by $\bM^{-1}$ transfers this property to the $\bM$-induced metric: for $\bv\in\calA(\bw)$ and $\widehat{\bv}\in\calA(\widehat{\bw})$,
\[
\ip{\bw-\widehat{\bw}}{\bM^{-1}\bv-\bM^{-1}\widehat{\bv}}_{\bM}
=\ip{\bw-\widehat{\bw}}{\bv-\widehat{\bv}}\geq0.
\]
The same identity transfers maximality, since any monotone extension of the graph of $\bM^{-1}\calA$ in this metric would induce a monotone extension of the graph of $\calA$. Thus $T_1$ is an everywhere-defined, single-valued resolvent.

To see its firm nonexpansiveness directly, let $\bx=T_1\bw$ and $\widehat{\bx}=T_1\widehat{\bw}$. The resolvent relations give
\[
\bM(\bw-\bx)\in\calA(\bx),
\qquad
\bM(\widehat{\bw}-\widehat{\bx})\in\calA(\widehat{\bx}).
\]
Monotonicity of $\calA$ then implies
\begin{equation}
\norm{T_1\bw-T_1\widehat{\bw}}_{\bM}^2
\leq\ip{T_1\bw-T_1\widehat{\bw}}{\bw-\widehat{\bw}}_{\bM}.
\label{eq:base-resolvent-firm}
\end{equation}
Expanding the squared norm shows that $2T_1-\calI$ is nonexpansive. Therefore, $T_1=\tfrac12\calI+\tfrac12(2T_1-\calI)$ is $1/2$-averaged.

\paragraph{Step 2: the forward map $T_2$ is averaged under the step-size condition.}

The composite loss has gradient $\bA^\top\nabla f(\bA\bbeta)$ and Lipschitz constant bounded by
\[
L:=L_f\norm{\bA}_2^2.
\]
We use the Schur complement of the lower-right block of $\bM$:
\begin{equation}
\bD_{\bM}:=\sigma^{-1}\bI_p-\tau\bK^\top\bK,
\qquad
s:=\lambda_{\min}(\bD_{\bM})=\sigma^{-1}-\tau\norm{\bK}_2^2.
\label{eq:base-schur-complement}
\end{equation}
Since $\tau>0$, we have $\bM\succ0$ if and only if $\bD_{\bM}\succ0$, equivalently $s>0$. The convergence argument below uses the condition $s>L/2$.

If $\bA=0$, then $\calS=0$ and $T_2=\calI$, so $T=T_1$ is already $1/2$-averaged. We therefore assume $\bA\neq0$ for the remainder of this step, which gives $L>0$.

Set $\calG:=\bM^{-1}\calS$. For $\bw=(\bbeta,\bnu)$ and $\widehat{\bw}=(\widehat{\bbeta},\widehat{\bnu})$, define
\[
\bd:=\bA^\top\bigl(\nabla f(\bA\bbeta)-\nabla f(\bA\widehat{\bbeta})\bigr).
\]
The gradient of a convex $L$-smooth function is $1/L$-cocoercive~\citep{bauschke2017convex}. Applied to $f\circ\bA$, this gives
\begin{equation}
\ip{\bbeta-\widehat{\bbeta}}{\bd}\geq\frac{1}{L}\norm{\bd}_2^2.
\label{eq:base-gradient-cocoercivity}
\end{equation}
The block inverse formula gives $(\bM^{-1})_{1:p,1:p}=\bD_{\bM}^{-1}$. Since $\calS(\bw)-\calS(\widehat{\bw})=(\bd,\vzero)$, we obtain
\begin{equation}
\begin{aligned}
\norm{\calG(\bw)-\calG(\widehat{\bw})}_{\bM}^2
&=\begin{bmatrix}\bd\\\vzero\end{bmatrix}^{\!\top}\bM^{-1}\begin{bmatrix}\bd\\\vzero\end{bmatrix}\\
&=\bd^\top\bD_{\bM}^{-1}\bd
\leq\frac{1}{s}\norm{\bd}_2^2.
\end{aligned}
\label{eq:base-forward-metric-bound}
\end{equation}
Combining Equations~\eqref{eq:base-gradient-cocoercivity} and~\eqref{eq:base-forward-metric-bound} gives
\begin{equation}
\begin{aligned}
\ip{\bw-\widehat{\bw}}{\calG(\bw)-\calG(\widehat{\bw})}_{\bM}
&=\ip{\bbeta-\widehat{\bbeta}}{\bd}\\
&\geq\frac{1}{L}\norm{\bd}_2^2\\
&\geq\frac{s}{L}\norm{\calG(\bw)-\calG(\widehat{\bw})}_{\bM}^2.
\end{aligned}
\label{eq:base-preconditioned-cocoercivity}
\end{equation}
Thus $\calG$ is $s/L$-cocoercive in the $\bM$-metric. Expanding the squared norm and using this inequality shows that $\calI-(2s/L)\calG$ is nonexpansive. Consequently,
\[
T_2=\calI-\calG
=(1-\alpha_2)\calI+\alpha_2\bigl(\calI-(2s/L)\calG\bigr),
\qquad
\alpha_2:=\frac{L}{2s},
\]
is $\alpha_2$-averaged whenever $s>L/2$. The inverses of $\bM$ and $\bD_{\bM}$ appear only in this analysis; Equation~\eqref{eq:base-cv-update} evaluates the iteration without forming them.

At the boundary $s=L/2>0$, the forward map $T_2$ is nonexpansive, since it then equals $\calI-(2s/L)\calG$. The resolvent $T_1$ is also nonexpansive, so their composition $T$ remains nonexpansive. This suffices for the pointwise residual estimates in Appendix~\ref{app:methodology-proofs}, but the convergence argument below requires the strict inequality $s>L/2$. If $L=0$, we still require $s>0$ for $\bM$ to define a norm.

\paragraph{Step 3: composition and convergence.}

For $L>0$, the composition of an $\alpha_1$-averaged operator and an $\alpha_2$-averaged operator is $\alpha$-averaged with~\citep{bauschke2017convex}
\begin{equation}
\alpha:=\frac{\alpha_1+\alpha_2-2\alpha_1\alpha_2}{1-\alpha_1\alpha_2}
=\frac{2s}{4s-L}\in(0,1),
\qquad
\alpha_1=\frac12,\quad\alpha_2=\frac{L}{2s}.
\label{eq:base-averaged-composition}
\end{equation}
For $L=0$, Step~2 instead gives $T=T_1$, and we take $\alpha=1/2$. In both cases, $T$ is averaged and therefore nonexpansive in the $\bM$-metric.

Let $\bw^\star$ be any saddle point, which is also a fixed point of $T$. Writing $T=(1-\alpha)\calI+\alpha\calR$ and using nonexpansiveness of $\calR$, the squared-norm identity for convex combinations gives
\begin{equation}
\norm{\bw^{t+1}-\bw^\star}_{\bM}^2
\leq\norm{\bw^t-\bw^\star}_{\bM}^2
-\frac{1-\alpha}{\alpha}\norm{\bw^{t+1}-\bw^t}_{\bM}^2.
\label{eq:base-fejer}
\end{equation}
Hence the distance to every fixed point is nonincreasing, and the iterates remain bounded. Summing Equation~\eqref{eq:base-fejer} over $t$ also gives
\begin{equation}
\sum_{t=0}^{\infty}\norm{\bw^{t+1}-\bw^t}_{\bM}^2
\leq\frac{\alpha}{1-\alpha}\norm{\bw^0-\bw^\star}_{\bM}^2<+\infty.
\label{eq:base-residual-summability}
\end{equation}
In particular, the fixed-point residual satisfies
\[
e^t:=\norm{(\calI-T)\bw^t}_{\bM}
=\norm{\bw^t-\bw^{t+1}}_{\bM}\longrightarrow0.
\]
Nonexpansiveness of $T$ also makes these residuals nonincreasing:
\[
e^{t+1}=\norm{T\bw^{t+1}-T\bw^t}_{\bM}
\leq\norm{\bw^{t+1}-\bw^t}_{\bM}=e^t.
\]
Consequently, Equation~\eqref{eq:base-residual-summability} yields the pointwise estimate
\begin{equation}
e^t\leq
\sqrt{\frac{\alpha}{(1-\alpha)(t+1)}}
\norm{\bw^0-\bw^\star}_{\bM}.
\label{eq:base-residual-pointwise-rate}
\end{equation}
Thus the exact fixed-step base iteration has $e^t=O((t+1)^{-1/2})$; the lower-bound errors inherit this rate whenever the corresponding assumptions of Theorem~\ref{theorem:convergence_rate} hold.
Because the product space is finite-dimensional, boundedness gives a convergent subsequence with limit $\overline{\bw}$. Continuity of $T$ and the vanishing residual imply $T\overline{\bw}=\overline{\bw}$. Applying Equation~\eqref{eq:base-fejer} with this fixed point shows that $\norm{\bw^t-\overline{\bw}}_{\bM}$ is nonincreasing; since it tends to zero along the subsequence, the entire sequence converges to $\overline{\bw}$. This limit satisfies Equation~\eqref{eq:base-zero-inclusion} and is therefore a saddle point.

We have thus proved convergence under the sufficient step-size condition
\begin{equation}
\sigma>0,\qquad\tau>0,\qquad
\sigma\tau\norm{\bK}_2^2+\frac{\sigma L_f\norm{\bA}_2^2}{2}<1,
\label{eq:base-cv-averaged-stepsizes}
\end{equation}
which is exactly $s>L/2$. For the stacked-identity operator used here, $\bK^\top\bK=(m+1)\bI_p$, so $\norm{\bK}_2^2=m+1$. Moreover, Equation~\eqref{eq:base-fejer} gives $\norm{\bw^t-\bw^\star}_{\bM}\leq\norm{\bw^0-\bw^\star}_{\bM}$ for every $t$. Together with $e^t\to0$, this establishes the boundedness and residual convergence used in Theorem~\ref{theorem:convergence_rate} for the fixed-step base iteration. The validity of the bounds and their error estimates still require the respective assumptions stated in that theorem and Appendix~\ref{app:dual-bounds}.
