# Supplementary material for: First-Order Primal-Dual Repairs for Scalable Branch and Bound
Source: arXiv:2610.26509 source file (2026-10-19)
Supplement: Supplementary file 4 [file C_accurqacy_and_convergence_db.tex]

\section{Convergence Analysis of the Dual Lower Bounds}
\label{app:methodology-proofs}

This appendix proves Theorem~\ref{theorem:convergence_rate}. We retain the notation of Appendices~\ref{sec:base-algorithm} and~\ref{app:dual-bounds} and fix a node $\calN$ throughout. The function $g$ is the original nonsmooth objective term, while $h$ collects the node-box indicator as block $0$ and the $m$ additional constraint indicators. Thus $\bK\bbeta=(\bbeta,\ldots,\bbeta)\in\mathbb R^{(m+1)p}$, and
\begin{align*}
p_{\calN}(\bbeta)&=f(\bA\bbeta)+g(\bbeta)+h(\bK\bbeta),\\
d(\bzeta,\bu,\bnu)&=-f^*(\bzeta)-g^*(\bu)-h^*(\bnu),\\
V(\bzeta,\bu,\bnu)&=\bA^\top\bzeta+\bu+\bK^\top\bnu.
\end{align*}
We assume that $f:\mathbb R^n\to\mathbb R$ is convex with an $L_f$-Lipschitz gradient, where $L_f>0$, and that $g$ and $h$ are proper, closed, and convex. All vector norms with subscript $2$ are Euclidean, and matrix norms with subscript $2$ are spectral norms.

The proof has three steps. First, we express the lower-bound errors through conjugate Bregman terms. Second, we bound the effect of the dual equality violation. Third, we relate both quantities to the fixed-point residual of one Condat--V\~u step. A finite lower bound requires finite conjugate values at the arguments where they are evaluated. The residual-corrected bound does not require the candidate tuple to satisfy the dual equality. Under the respective assumptions of Theorem~\ref{theorem:convergence_rate}, the certificate errors are $O(e^t)$ as $e^t\to0$, so they inherit residual-rate upper bounds.

We use the main-text notation $\bz^t=(\bbeta^t,\bnu^t)$ and $\bz^\star=(\bbeta^\star,\bnu^\star)$. The matrix $M=\bM$ and the fixed Condat--V\~u map $T$ are defined in Appendix~\ref{sec:base-algorithm}. Set
\[
L:=L_f\norm{\bA}_2^2,\qquad
s:=\sigma^{-1}-\tau\norm{\bK}_2^2>0,\qquad s\geq L/2.
\]
The strict positivity of $s$ ensures that $M$ defines a norm and that the constants containing $1/s$ are defined. The positive boundary $s=L/2$ is sufficient for the pointwise estimates; convergence of the fixed-step base iteration uses $s>L/2$, as established in Appendix~\ref{sec:base-cv-convergence}.

At a fixed monitored iteration $t$, Algorithm~\ref{alg:compute_safe_lower_bound} constructs
\begin{align*}
\bz^{t,+}=\bz^+&=(\bbeta^+,\bnu^+):=T\bz^t,\qquad
\bzeta^+:=\nabla f(\bA\bbeta^t),\\
\bu^+&:=\sigma^{-1}(\bbeta^t-\bbeta^+)-\bA^\top\bzeta^+-\bK^\top\bnu^t,\\
\widetilde{\bu}&:=-\bA^\top\bzeta^+-\bK^\top\bnu^+,\qquad
\br^t:=\bz^t-\bz^+,\qquad e^t:=\norm{\br^t}_M.
\end{align*}
We denote this reconstructed dual tuple by $Q(\bz^t):=(\bzeta^+,\bu^+,\bnu^+)$ and evaluate every lower bound and Bregman term in the statements below at this same tuple (with $\bu^+$ replaced by $\widetilde{\bu}$ for the repaired bound). As in Theorem~\ref{theorem:convergence_rate},
\[
\Delta_{\mathrm{repair}}(\bz^t):=d^\star-\mathrm{LB}_{\mathrm{repair}}^t,
\qquad
\Delta_{\mathrm{violation}}(\bz^t):=d^\star-\mathrm{LB}_{\mathrm{violation}}^t.
\]
Let the primal--dual optimal pair satisfy the saddle-point conditions
\begin{equation}
\bzeta^\star=\nabla f(\bA\bbeta^\star),\quad
\bu^\star\in\partial g(\bbeta^\star),\quad
\bnu^\star\in\partial h(\bK\bbeta^\star),\quad
V(\bzeta^\star,\bu^\star,\bnu^\star)=\vzero.
\label{eq:lower-bound-kkt-app}
\end{equation}
These conditions follow from the saddle solution in Theorem~\ref{theorem:convergence_rate} and imply $d^\star=p_{\calN}^\star$. The next three statements restate the main-text lemmas in this common notation.

\subsection{Valid Lower Bounds}
\begin{restated}{Lemma~\ref{lemma:lower_bounds_are_valid} (Valid Lower Bounds)}
Let $\bbeta^\star$ and $(\bzeta^\star,\bu^\star,\bnu^\star)$ be a pair of primal--dual optimal solutions, with the saddle-point conditions specified above. Define the conjugate Bregman terms as
\begin{align*}
B_f(\bzeta)&:=f^*(\bzeta)-f^*(\bzeta^\star)-\ip{\bA\bbeta^\star}{\bzeta-\bzeta^\star},\\
B_g(\bu)&:=g^*(\bu)-g^*(\bu^\star)-\ip{\bbeta^\star}{\bu-\bu^\star},\\
B_h(\bnu)&:=h^*(\bnu)-h^*(\bnu^\star)-\ip{\bK\bbeta^\star}{\bnu-\bnu^\star},\\
B(\bzeta,\bu,\bnu)&:=B_f(\bzeta)+B_g(\bu)+B_h(\bnu).
\end{align*}
These terms are nonnegative. For Algorithm~\ref{alg:compute_safe_lower_bound}, the repaired lower bound satisfies
\[
\Delta_{\mathrm{repair}}(\bz^t)=B(\bzeta^+,\widetilde{\bu},\bnu^+)\geq0.
\]
Under Assumption~2 of Theorem~\ref{theorem:convergence_rate},
\[
\Delta_{\mathrm{violation}}(\bz^t)
=B(\bzeta^+,\bu^+,\bnu^+)
+\sigma_{\calD-\bbeta^\star}\!\left(-V(\bzeta^+,\bu^+,\bnu^+)\right)\geq0,
\]
where $\calD-\bbeta^\star:=\{\bbeta-\bbeta^\star:\bbeta\in\calD\}$.
\end{restated}

The repaired error is finite when $g^*(\widetilde{\bu})$ is finite, as guaranteed by Assumption~1 of the theorem; otherwise the identity holds with value $+\infty$. The proof establishes the identities for a generic tuple and then applies them to $Q(\bz^t)$.

\begin{proof}
For a generic tuple $(\bzeta,\bu,\bnu)$ with finite conjugate values, set $\widetilde{\bu}:=-\bA^\top\bzeta-\bK^\top\bnu$.
Since $f$, $g$, and $h$ are proper, closed, and convex functions, the KKT conditions also give
\begin{align}
\bA\bbeta^\star\in\partial f^*(\bzeta^\star),
\qquad
\bbeta^\star\in\partial g^*(\bu^\star),
\qquad
\bK\bbeta^\star\in\partial h^*(\bnu^\star).
\end{align}
Since $f^*$ is convex, the first inclusion gives
\begin{equation}
f^*(\bzeta)\geq f^*(\bzeta^\star)
+\ip{\bA\bbeta^\star}{\bzeta-\bzeta^\star},
\end{equation}
so $B_f(\bzeta)\geq0$. The same argument gives $B_g(\bu)\geq0$ and $B_h(\bnu)\geq0$.

The KKT conditions imply equality in the three Fenchel--Young inequalities:
\begin{align*}
f(\bA\bbeta^\star)+f^*(\bzeta^\star)
&=\ip{\bA\bbeta^\star}{\bzeta^\star},\\
g(\bbeta^\star)+g^*(\bu^\star)
&=\ip{\bbeta^\star}{\bu^\star},\\
h(\bK\bbeta^\star)+h^*(\bnu^\star)
&=\ip{\bK\bbeta^\star}{\bnu^\star}.
\end{align*}
Adding these identities gives
\[
p_{\calN}(\bbeta^\star)-d(\bzeta^\star,\bu^\star,\bnu^\star)
=\ip{\bbeta^\star}{V(\bzeta^\star,\bu^\star,\bnu^\star)}
=0.
\]
Weak duality then yields
\[
d(\bzeta^\star,\bu^\star,\bnu^\star)
\leq d^\star
\leq p_{\calN}^\star
\leq p_{\calN}(\bbeta^\star)
=d(\bzeta^\star,\bu^\star,\bnu^\star).
\]
Hence $d^\star=p_{\calN}^\star$, and the KKT tuple attains both optima.

Expanding the definition of $B$ gives
\begin{align*}
B(\bzeta,\bu,\bnu)
&=\bigl[f^*(\bzeta)+g^*(\bu)+h^*(\bnu)\bigr]
-\bigl[f^*(\bzeta^\star)+g^*(\bu^\star)+h^*(\bnu^\star)\bigr]\\
&\quad-\ip{\bbeta^\star}{\bA^\top\bzeta+\bu+\bK^\top\bnu}
+\ip{\bbeta^\star}{\bA^\top\bzeta^\star+\bu^\star+\bK^\top\bnu^\star}\\
&=-d(\bzeta,\bu,\bnu)+d^\star
-\ip{\bbeta^\star}{V(\bzeta,\bu,\bnu)},
\end{align*}
where we used $d(\bzeta^\star,\bu^\star,\bnu^\star)=d^\star$ and $V(\bzeta^\star,\bu^\star,\bnu^\star)=\vzero$.

For the repair construction, $V(\bzeta,\widetilde{\bu},\bnu)=\vzero$ by definition of $\widetilde{\bu}$. Substituting $(\bzeta,\widetilde{\bu},\bnu)$ into the preceding identity therefore yields
\begin{align}
d^\star-\mathrm{LB}_{\mathrm{repair}}(\bzeta,\bu,\bnu)
=d^\star-d(\bzeta,\widetilde{\bu},\bnu)
=B(\bzeta,\widetilde{\bu},\bnu)\geq0.
\end{align}

For the violation construction, the same identity and the definition of the support function give
\begin{align*}
d^\star-\mathrm{LB}_{\mathrm{violation}}(\bzeta,\bu,\bnu)
&=d^\star-d(\bzeta,\bu,\bnu)
+\sigma_{\calD}\!\left(-V(\bzeta,\bu,\bnu)\right)\\
&=d^\star-d(\bzeta,\bu,\bnu)
+\sup_{\bbeta\in\calD}\ip{\bbeta}{-V(\bzeta,\bu,\bnu)}\\
&=B(\bzeta,\bu,\bnu)
+\ip{\bbeta^\star}{V(\bzeta,\bu,\bnu)}
+\sup_{\bbeta\in\calD}\ip{\bbeta}{-V(\bzeta,\bu,\bnu)}\\
&=B(\bzeta,\bu,\bnu)
+\sup_{\bbeta\in\calD}\ip{\bbeta^\star-\bbeta}{V(\bzeta,\bu,\bnu)}\\
&=B(\bzeta,\bu,\bnu)
+\sigma_{\calD-\bbeta^\star}\!\left(-V(\bzeta,\bu,\bnu)\right)
\geq0.
\end{align*}
The last inequality follows because $B(\bzeta,\bu,\bnu)\geq0$ and $\bbeta^\star\in\dom p_{\calN}\subseteq\calD$, so the supremum is at least its value $0$ at $\bbeta=\bbeta^\star$.
\end{proof}

The preceding identities involve either the repaired argument $\widetilde{\bu}$ or a support-function correction. The next lemma bounds their contributions using the uncorrected Bregman terms and the norm of the dual equality violation.

\subsection{Surrogate Lower Bounds}
\begin{restated}{Lemma~\ref{lemma:surrogate_lower_bounds} (Surrogate Lower Bounds)}
Let $\bbeta^\star$ and $B$ be as in Lemma~\ref{lemma:lower_bounds_are_valid}, and let $(\bzeta^+,\bu^+,\bnu^+)$ be the tuple constructed by Algorithm~\ref{alg:compute_safe_lower_bound} at $\bz^t$. Under Assumption~1 of Theorem~\ref{theorem:convergence_rate}, namely that $g^*$ is $L_{g^*}$-Lipschitz,
\[
\Delta_{\mathrm{repair}}(\bz^t)
\leq B(\bzeta^+,\bu^+,\bnu^+)
+C_{\mathrm{repair}}\norm{V(\bzeta^+,\bu^+,\bnu^+)}_2,
\qquad C_{\mathrm{repair}}:=L_{g^*}+\norm{\bbeta^\star}_2.
\]
Under Assumption~2 of the theorem, namely that $\calD$ is nonempty, compact, and convex and contains $\dom p_{\calN}$,
\[
\Delta_{\mathrm{violation}}(\bz^t)
\leq B(\bzeta^+,\bu^+,\bnu^+)
+R_{\bbeta}\norm{V(\bzeta^+,\bu^+,\bnu^+)}_2,
\qquad R_{\bbeta}:=\sup_{\bbeta\in\calD}\norm{\bbeta-\bbeta^\star}_2.
\]
\end{restated}

\begin{proof}
We prove the estimates for a generic finite-conjugate tuple $(\bzeta,\bu,\bnu)$, with $\widetilde{\bu}:=-\bA^\top\bzeta-\bK^\top\bnu$; substituting $Q(\bz^t)$ gives the stated inequalities.
For the repair construction, Lemma~\ref{lemma:lower_bounds_are_valid} and the definition of $B_g$ give
\begin{align*}
d^\star-\mathrm{LB}_{\mathrm{repair}}(\bzeta,\bu,\bnu)
&=B(\bzeta,\widetilde{\bu},\bnu)\\
&=B(\bzeta,\bu,\bnu)+B_g(\widetilde{\bu})-B_g(\bu)\\
&=B(\bzeta,\bu,\bnu)
+g^*(\widetilde{\bu})-g^*(\bu)
-\ip{\bbeta^\star}{\widetilde{\bu}-\bu}.
\end{align*}
Note that
\begin{equation}
\widetilde{\bu}
=-\bA^\top\bzeta-\bK^\top\bnu
=\bu-\bigl(\bA^\top\bzeta+\bu+\bK^\top\bnu\bigr)
=\bu-V(\bzeta,\bu,\bnu).
\end{equation}
Substituting this identity yields
\begin{align*}
d^\star-\mathrm{LB}_{\mathrm{repair}}(\bzeta,\bu,\bnu)
&=B(\bzeta,\bu,\bnu)
+g^*\!\left(\bu-V(\bzeta,\bu,\bnu)\right)-g^*(\bu)\\
&\quad+\ip{\bbeta^\star}{V(\bzeta,\bu,\bnu)}.
\end{align*}
Under Assumption~1, the global Lipschitz continuity of $g^*$ gives
\begin{equation}
g^*\!\left(\bu-V(\bzeta,\bu,\bnu)\right)-g^*(\bu)
\leq
\left|g^*\!\left(\bu-V(\bzeta,\bu,\bnu)\right)-g^*(\bu)\right|
\leq
L_{g^*}\norm{V(\bzeta,\bu,\bnu)}_2.
\end{equation}
Also, by the Cauchy--Schwarz inequality,
\begin{equation}
\ip{\bbeta^\star}{V(\bzeta,\bu,\bnu)}
\leq
\left|\ip{\bbeta^\star}{V(\bzeta,\bu,\bnu)}\right|
\leq
\norm{\bbeta^\star}_2\norm{V(\bzeta,\bu,\bnu)}_2.
\end{equation}
Combining these two inequalities proves the repair bound.

For the violation construction, Lemma~\ref{lemma:lower_bounds_are_valid} and the Cauchy--Schwarz inequality give
\begin{align*}
d^\star-\mathrm{LB}_{\mathrm{violation}}(\bzeta,\bu,\bnu)
&=B(\bzeta,\bu,\bnu)
+\sup_{\bbeta\in\calD}\ip{\bbeta^\star-\bbeta}{V(\bzeta,\bu,\bnu)}\\
&\leq B(\bzeta,\bu,\bnu)
+\sup_{\bbeta\in\calD}
\norm{\bbeta^\star-\bbeta}_2
\norm{V(\bzeta,\bu,\bnu)}_2\\
&=B(\bzeta,\bu,\bnu)
+R_{\bbeta}\norm{V(\bzeta,\bu,\bnu)}_2.
\end{align*}
\end{proof}

We now evaluate the quantities in Lemma~\ref{lemma:surrogate_lower_bounds} at the dual tuple reconstructed from one Condat--V\~u step. This connects the lower-bound error to the fixed-point residual without assuming that the input was generated by the base iteration.

\subsection{One-step Bregman Estimate}
\begin{restated}{Lemma~\ref{lemma:one_step_Bregman_estimate} (One-step Bregman Estimate)}
Let $\bz^+=(\bbeta^+,\bnu^+)=T\bz^t$, $\br^t=\bz^t-\bz^+$, and $\br_{\bbeta}^t=\bbeta^t-\bbeta^+$. Set $L:=L_f\norm{\bA}_2^2$. Then the following estimates hold:
\begin{enumerate}[label=(\alph*)]
\item The dual equality violation satisfies
\begin{equation}
\norm{V(\bzeta^+,\bu^+,\bnu^+)}_2
\leq\frac{1}{\sqrt{\sigma}}\norm{\br^t}_M.
\label{eq:one-step-violation-estimate-app}
\end{equation}
\item The conjugate Bregman terms satisfy
\begin{equation}
B(\bzeta^+,\bu^+,\bnu^+)
\leq\frac12\left(\norm{\bz^t-\bz^\star}_M^2
-\norm{\bz^+-\bz^\star}_M^2-\norm{\br^t}_M^2\right)
+\frac{L}{2}\norm{\br_{\bbeta}^t}_2^2.
\label{eq:one-step-bregman-estimate-app}
\end{equation}
\item If $\norm{\bz^t-\bz^\star}_M\leq R_{\bz}$, then
\begin{equation}
B(\bzeta^+,\bu^+,\bnu^+)
\leq R_{\bz}e^t+\frac{L_f\norm{\bA}_2^2}{2s}(e^t)^2.
\label{eq:one-step-bregman-residual-estimate-app}
\end{equation}
\end{enumerate}
\end{restated}

\begin{proof}
For this proof we suppress the iteration index: $\bz=\bz^t=(\bbeta,\bnu)$, $\br=\br^t$, and $e=e^t$. Thus $\bz^+=T\bz$ and $\bz^\star=(\bbeta^\star,\bnu^\star)$ throughout.
We first verify that the conjugates evaluated at $Q(\bz)$ are finite. Since $\bzeta^+=\nabla f(\bA\bbeta)$, Fenchel--Young equality gives
\[
f^*(\bzeta^+)
=\ip{\bzeta^+}{\bA\bbeta}-f(\bA\bbeta)
<+\infty.
\]
The primal proximal optimality condition gives $\bu^+\in\partial g(\bbeta^+)$, so
\[
g^*(\bu^+)
=\ip{\bu^+}{\bbeta^+}-g(\bbeta^+)
<+\infty.
\]
The dual proximal optimality condition gives
\[
\bK(2\bbeta^+-\bbeta)
+\frac{\bnu-\bnu^+}{\tau}
\in\partial h^*(\bnu^+),
\]
which implies $\bnu^+\in\dom h^*$. We derive these two proximal optimality conditions explicitly in part~(b).

\textit{(a) Bounding the dual equality violation.}
By the definition of $\bu^+$,
\begin{align*}
V(\bzeta^+,\bu^+,\bnu^+)
&=\bA^\top\bzeta^++\bu^++\bK^\top\bnu^+\\
&=\frac{\bbeta-\bbeta^+}{\sigma}
-\bK^\top(\bnu-\bnu^+)\\
&=\begin{bmatrix}\bI_p&0\end{bmatrix}\bM\br,
\end{align*}
where
\[
\bM=
\begin{bmatrix}
\sigma^{-1}\bI_p&-\bK^\top\\
-\bK&\tau^{-1}\bI_{(m+1)p}
\end{bmatrix}.
\]
It remains to bound $\norm{\begin{bmatrix}\bI_p&0\end{bmatrix}\bM\br}_2$.

For any $\ba\in\mathbb R^p$ with $\norm{\ba}_2=1$, the definition of $\bM$ gives
\begin{equation}
\left\|
\begin{bmatrix}\ba\\\vzero\end{bmatrix}
\right\|_{\bM}^2
=
\begin{bmatrix}\ba\\\vzero\end{bmatrix}^{\!\top}
\bM
\begin{bmatrix}\ba\\\vzero\end{bmatrix}
=
\frac1\sigma\norm{\ba}_2^2
=
\frac1\sigma.
\end{equation}
Using the dual representation of the Euclidean norm and the Cauchy--Schwarz inequality for the $\bM$-induced inner product, we obtain
\begin{align*}
\norm{V(\bzeta^+,\bu^+,\bnu^+)}_2
&=\sup_{\norm{\ba}_2=1}
\left|\ip{\ba}{V(\bzeta^+,\bu^+,\bnu^+)}\right|\\
&=\sup_{\norm{\ba}_2=1}
\left|\ip{\ba}{\begin{bmatrix}\bI_p&0\end{bmatrix}\bM\br}\right|\\
&=\sup_{\norm{\ba}_2=1}
\left|
\left\langle
\begin{bmatrix}\ba\\\vzero\end{bmatrix},
\br
\right\rangle_{\bM}
\right|\\
&\leq
\sup_{\norm{\ba}_2=1}
\left\|
\begin{bmatrix}\ba\\\vzero\end{bmatrix}
\right\|_{\bM}
\norm{\br}_{\bM}\\
&=\frac1{\sqrt{\sigma}}\norm{\br}_{\bM}.
\end{align*}

\textit{(b) Deriving the one-step Bregman estimate.}
We first bound $B_g(\bu^+)$ and $B_h(\bnu^+)$ using the two proximal updates. The primal update and the definition of $\bu^+$ give
\begin{equation}
\bbeta^+
=
\prox_{\sigma g}\!\left(
\bbeta-\sigma\bA^\top\nabla f(\bA\bbeta)-\sigma\bK^\top\bnu
\right)
=
\prox_{\sigma g}(\bbeta^++\sigma\bu^+).
\end{equation}
The optimality condition for this proximal problem is
\begin{equation}
\vzero
\in
\bbeta^+-(\bbeta^++\sigma\bu^+)
+\sigma\partial g(\bbeta^+),
\end{equation}
so $\bu^+\in\partial g(\bbeta^+)$, or equivalently $\bbeta^+\in\partial g^*(\bu^+)$. The subgradient inequality for $g^*$ at $\bu^+$ therefore gives
\begin{equation}
g^*(\bu^\star)
\geq
g^*(\bu^+)+\ip{\bbeta^+}{\bu^\star-\bu^+},
\end{equation}
or equivalently
\begin{equation}
g^*(\bu^+)-g^*(\bu^\star)
\leq
\ip{\bbeta^+}{\bu^+-\bu^\star}.
\end{equation}
Subtracting $\ip{\bbeta^\star}{\bu^+-\bu^\star}$ from both sides and using the definition of $B_g$, we obtain
\begin{equation}
B_g(\bu^+)
\leq
\ip{\bbeta^+-\bbeta^\star}{\bu^+-\bu^\star}.
\label{eq:one-step-g-bregman-bound-app}
\end{equation}

Similarly, the dual update gives
\begin{equation}
\bnu^+
=
\prox_{\tau h^*}\!\left(
\bnu+\tau\bK(2\bbeta^+-\bbeta)
\right),
\end{equation}
or equivalently
\begin{equation}
\vzero
\in
\bnu^+
-\left(\bnu+\tau\bK(2\bbeta^+-\bbeta)\right)
+\tau\partial h^*(\bnu^+).
\end{equation}
Rearranging this optimality condition gives
\begin{equation}
\bK(2\bbeta^+-\bbeta)
+\frac{\bnu-\bnu^+}{\tau}
\in\partial h^*(\bnu^+).
\end{equation}
The subgradient inequality for $h^*$ at $\bnu^+$ therefore gives
\begin{equation}
h^*(\bnu^\star)
\geq
h^*(\bnu^+)
+
\left\langle
\bK(2\bbeta^+-\bbeta)+\frac{\bnu-\bnu^+}{\tau},
\bnu^\star-\bnu^+
\right\rangle,
\end{equation}
or equivalently
\begin{equation}
h^*(\bnu^+)-h^*(\bnu^\star)
\leq
\left\langle
\bK(2\bbeta^+-\bbeta)+\frac{\bnu-\bnu^+}{\tau},
\bnu^+-\bnu^\star
\right\rangle.
\end{equation}
Subtracting $\ip{\bK\bbeta^\star}{\bnu^+-\bnu^\star}$ from both sides and using the definition of $B_h$, we obtain
\begin{equation}
\begin{aligned}
B_h(\bnu^+)
&=h^*(\bnu^+)-h^*(\bnu^\star)
-\ip{\bK\bbeta^\star}{\bnu^+-\bnu^\star}\\
&\leq
\left\langle
\bK(2\bbeta^+-\bbeta)
+\frac{\bnu-\bnu^+}{\tau}
-\bK\bbeta^\star,
\bnu^+-\bnu^\star
\right\rangle.
\end{aligned}
\label{eq:one-step-h-bregman-bound-app}
\end{equation}

We now combine the bounds on $B_g(\bu^+)$ and $B_h(\bnu^+)$. We first rewrite each right-hand side using the residual components
\begin{equation}
\br_{\bbeta}=\bbeta-\bbeta^+,
\qquad
\br_{\bnu}=\bnu-\bnu^+.
\end{equation}

For the bound on $B_g(\bu^+)$, recall that
\begin{equation}
\bu^+
=
\frac{\bbeta-\bbeta^+}{\sigma}
-\bA^\top\bzeta^+-\bK^\top\bnu,
\qquad
\bu^\star
=
-\bA^\top\bzeta^\star-\bK^\top\bnu^\star,
\end{equation}
where the second equality is the KKT equality at the optimal solution. Subtracting these two expressions gives
\begin{align*}
\bu^+-\bu^\star
&=
\frac{\bbeta-\bbeta^+}{\sigma}
-\bA^\top\bzeta^+-\bK^\top\bnu
+\bA^\top\bzeta^\star+\bK^\top\bnu^\star\\
&=
\frac{\br_{\bbeta}}{\sigma}
-\bA^\top(\bzeta^+-\bzeta^\star)
-\bK^\top(\bnu-\bnu^\star).
\end{align*}
The last difference can be split as
\begin{equation}
\bnu-\bnu^\star
=
(\bnu-\bnu^+)+(\bnu^+-\bnu^\star)
=
\br_{\bnu}+(\bnu^+-\bnu^\star).
\end{equation}
Substituting this identity into the preceding expression yields
\begin{equation}
\bu^+-\bu^\star
=
\left(
\frac{\br_{\bbeta}}{\sigma}-\bK^\top\br_{\bnu}
\right)
-\bK^\top(\bnu^+-\bnu^\star)
-\bA^\top(\bzeta^+-\bzeta^\star).
\end{equation}
We can now substitute into Equation~\eqref{eq:one-step-g-bregman-bound-app} and distribute the inner product:
\begin{align*}
B_g(\bu^+)
&\leq
\ip{\bbeta^+-\bbeta^\star}{\bu^+-\bu^\star}\\
&=
\left\langle
\bbeta^+-\bbeta^\star,
\frac{\br_{\bbeta}}{\sigma}-\bK^\top\br_{\bnu}
\right\rangle\\
&\quad-
\ip{\bbeta^+-\bbeta^\star}{\bK^\top(\bnu^+-\bnu^\star)}\\
&\quad-
\ip{\bbeta^+-\bbeta^\star}{\bA^\top(\bzeta^+-\bzeta^\star)}.
\end{align*}

For the bound on $B_h(\bnu^+)$, first observe that
\begin{equation}
2\bbeta^+-\bbeta-\bbeta^\star
=
(\bbeta^+-\bbeta^\star)-(\bbeta-\bbeta^+)
=
(\bbeta^+-\bbeta^\star)-\br_{\bbeta}.
\end{equation}
Using this identity and $\bnu-\bnu^+=\br_{\bnu}$, the first argument of the inner product in Equation~\eqref{eq:one-step-h-bregman-bound-app} becomes
\begin{align*}
\bK(2\bbeta^+-\bbeta)
+\frac{\bnu-\bnu^+}{\tau}
-\bK\bbeta^\star
&=
\bK(2\bbeta^+-\bbeta-\bbeta^\star)
+\frac{\br_{\bnu}}{\tau}\\
&=
\bK(\bbeta^+-\bbeta^\star)
-\bK\br_{\bbeta}
+\frac{\br_{\bnu}}{\tau}.
\end{align*}
Substituting into that bound and distributing the inner product gives
\begin{align*}
B_h(\bnu^+)
&\leq
\left\langle
\bK(\bbeta^+-\bbeta^\star)
-\bK\br_{\bbeta}
+\frac{\br_{\bnu}}{\tau},
\bnu^+-\bnu^\star
\right\rangle\\
&=
\ip{\bK(\bbeta^+-\bbeta^\star)}{\bnu^+-\bnu^\star}
+
\left\langle
\frac{\br_{\bnu}}{\tau}-\bK\br_{\bbeta},
\bnu^+-\bnu^\star
\right\rangle.
\end{align*}

We now add the two expanded bounds. The bound on $B_g(\bu^+)$ contains a negative coupling term, while the bound on $B_h(\bnu^+)$ contains its positive counterpart. They cancel because $\ip{\ba}{\bK^\top\bb}=\ip{\bK\ba}{\bb}$:
\begin{align*}
&-\ip{\bbeta^+-\bbeta^\star}{\bK^\top(\bnu^+-\bnu^\star)}
+\ip{\bK(\bbeta^+-\bbeta^\star)}{\bnu^+-\bnu^\star}\\
&\qquad=
-\ip{\bK(\bbeta^+-\bbeta^\star)}{\bnu^+-\bnu^\star}
+\ip{\bK(\bbeta^+-\bbeta^\star)}{\bnu^+-\bnu^\star}
=0.
\end{align*}
After this cancellation, we obtain
\begin{align*}
B_g(\bu^+)+B_h(\bnu^+)
&\leq
\left\langle
\bbeta^+-\bbeta^\star,
\frac{\br_{\bbeta}}{\sigma}-\bK^\top\br_{\bnu}
\right\rangle\\
&\quad+
\left\langle
\bnu^+-\bnu^\star,
\frac{\br_{\bnu}}{\tau}-\bK\br_{\bbeta}
\right\rangle\\
&\quad-
\ip{\bbeta^+-\bbeta^\star}{\bA^\top(\bzeta^+-\bzeta^\star)}.
\end{align*}

It remains to express the first two terms using the $\bM$-induced inner product. By the definitions of $\bM$ and $\br$,
\begin{equation}
\bM\br
=
\begin{bmatrix}
\sigma^{-1}\bI_p&-\bK^\top\\
-\bK&\tau^{-1}\bI_{(m+1)p}
\end{bmatrix}
\begin{bmatrix}
\br_{\bbeta}\\
\br_{\bnu}
\end{bmatrix}
=
\begin{bmatrix}
\sigma^{-1}\br_{\bbeta}-\bK^\top\br_{\bnu}\\
\tau^{-1}\br_{\bnu}-\bK\br_{\bbeta}
\end{bmatrix}.
\end{equation}
Since $\bz^+-\bz^\star=(\bbeta^+-\bbeta^\star,\bnu^+-\bnu^\star)$, this gives
\begin{align*}
\ip{\bz^+-\bz^\star}{\br}_{\bM}
&=
\ip{\bz^+-\bz^\star}{\bM\br}\\
&=
\left\langle
\bbeta^+-\bbeta^\star,
\frac{\br_{\bbeta}}{\sigma}-\bK^\top\br_{\bnu}
\right\rangle\\
&\quad+
\left\langle
\bnu^+-\bnu^\star,
\frac{\br_{\bnu}}{\tau}-\bK\br_{\bbeta}
\right\rangle.
\end{align*}
Also,
\begin{equation}
\ip{\bbeta^+-\bbeta^\star}{\bA^\top(\bzeta^+-\bzeta^\star)}
=
\ip{\bA(\bbeta^+-\bbeta^\star)}{\bzeta^+-\bzeta^\star}.
\end{equation}
Substituting these two identities into the bound on the sum yields
\begin{equation}
B_g(\bu^+)+B_h(\bnu^+)
\leq
\ip{\bz^+-\bz^\star}{\br}_{\bM}
-
\ip{\bA(\bbeta^+-\bbeta^\star)}{\bzeta^+-\bzeta^\star}.
\end{equation}
We now add $B_f(\bzeta^+)$ to the bound on $B_g(\bu^+)+B_h(\bnu^+)$. Recall that
\begin{equation}
B_f(\bzeta^+)
=
f^*(\bzeta^+)-f^*(\bzeta^\star)
-\ip{\bA\bbeta^\star}{\bzeta^+-\bzeta^\star}.
\end{equation}
By the definition of $B$ and the preceding bound,
\begin{align*}
B(\bzeta^+,\bu^+,\bnu^+)
&=
B_f(\bzeta^+)
+\bigl(B_g(\bu^+)+B_h(\bnu^+)\bigr)\\
&\leq
B_f(\bzeta^+)
+\ip{\bz^+-\bz^\star}{\br}_{\bM}
-\ip{\bA(\bbeta^+-\bbeta^\star)}{\bzeta^+-\bzeta^\star}\\
&=
\ip{\bz^+-\bz^\star}{\br}_{\bM}
+f^*(\bzeta^+)-f^*(\bzeta^\star)\\
&\quad-
\ip{\bA\bbeta^\star}{\bzeta^+-\bzeta^\star}
-\ip{\bA(\bbeta^+-\bbeta^\star)}{\bzeta^+-\bzeta^\star}.
\end{align*}
The last two inner products have the same second argument. By linearity, they combine as
\begin{align*}
&-\ip{\bA\bbeta^\star}{\bzeta^+-\bzeta^\star}
-\ip{\bA(\bbeta^+-\bbeta^\star)}{\bzeta^+-\bzeta^\star}\\
&\qquad=
-\ip{\bA\bbeta^\star+\bA(\bbeta^+-\bbeta^\star)}{\bzeta^+-\bzeta^\star}\\
&\qquad=
-\ip{\bA\bbeta^+}{\bzeta^+-\bzeta^\star},
\end{align*}
where the last equality uses $\bA\bbeta^\star+\bA(\bbeta^+-\bbeta^\star)=\bA\bbeta^+$. Substituting this identity into the bound above gives
\begin{align}
B(\bzeta^+,\bu^+,\bnu^+)
&\leq
\ip{\bz^+-\bz^\star}{\br}_{\bM}
+f^*(\bzeta^+)-f^*(\bzeta^\star)
-\ip{\bA\bbeta^+}{\bzeta^+-\bzeta^\star}.
\label{eq:one-step-bregman-before-smoothness-app}
\end{align}

We next bound the terms involving $f^*$. Since $f:\mathbb R^n\to\mathbb R$ is convex and $L_f$-smooth, its conjugate $f^*$ is $1/L_f$-strongly convex~\citep{bauschke2017convex}. Moreover, $\bzeta^+=\nabla f(\bA\bbeta)$ implies $\bA\bbeta\in\partial f^*(\bzeta^+)$. Hence,
\begin{equation}
f^*(\bzeta^\star)
\geq
f^*(\bzeta^+)
+\ip{\bA\bbeta}{\bzeta^\star-\bzeta^+}
+\frac1{2L_f}\norm{\bzeta^\star-\bzeta^+}_2^2.
\end{equation}
Using this inequality and completing the square, we obtain
\begin{align*}
&f^*(\bzeta^+)-f^*(\bzeta^\star)
-\ip{\bA\bbeta^+}{\bzeta^+-\bzeta^\star}\\
&\quad=
f^*(\bzeta^+)-f^*(\bzeta^\star)
+\ip{\bA\bbeta}{\bzeta^\star-\bzeta^+}
+\ip{\bA(\bbeta^+-\bbeta)}{\bzeta^\star-\bzeta^+}\\
&\quad\leq
-\frac1{2L_f}\norm{\bzeta^\star-\bzeta^+}_2^2
+\ip{\bA(\bbeta^+-\bbeta)}{\bzeta^\star-\bzeta^+}\\
&\quad=
-\frac1{2L_f}
\norm{\bzeta^\star-\bzeta^+-L_f\bA(\bbeta^+-\bbeta)}_2^2
+\frac{L_f}{2}\norm{\bA(\bbeta^+-\bbeta)}_2^2\\
&\quad\leq
\frac{L_f}{2}\norm{\bA(\bbeta^+-\bbeta)}_2^2\\
&\quad\leq
\frac{L_f\norm{\bA}_2^2}{2}\norm{\br_{\bbeta}}_2^2
=
\frac{L}{2}\norm{\br_{\bbeta}}_2^2.
\end{align*}
Substituting into Equation~\eqref{eq:one-step-bregman-before-smoothness-app} yields
\begin{equation}
B(\bzeta^+,\bu^+,\bnu^+)
\leq
\ip{\bz^+-\bz^\star}{\br}_{\bM}
+\frac{L}{2}\norm{\br_{\bbeta}}_2^2.
\label{eq:one-step-bregman-inner-product-app}
\end{equation}
Finally, since $\bz-\bz^\star=\br+(\bz^+-\bz^\star)$,
\begin{equation}
\norm{\bz-\bz^\star}_{\bM}^2
=
\norm{\br}_{\bM}^2
+\norm{\bz^+-\bz^\star}_{\bM}^2
+2\ip{\bz^+-\bz^\star}{\br}_{\bM}.
\end{equation}
We prove part~(b) by rearranging this equality to obtain an expression for $\ip{\bz^+-\bz^\star}{\br}_{\bM}$ and substituting it into Equation~\eqref{eq:one-step-bregman-inner-product-app}.

\textit{(c) Expressing the estimate in terms of the residual norm.}
Recall that from part~(b), we have
\begin{equation}
B(\bzeta^+,\bu^+,\bnu^+)
\leq
\ip{\bz^+-\bz^\star}{\br}_{\bM}
+\frac{L}{2}\norm{\br_{\bbeta}}_2^2.
\label{eq:one-step-bregman-inner-product_part_c-app}
\end{equation}
We bound the two terms separately.

Under the stated step-size condition, $T$ is nonexpansive in the $\bM$-norm, as shown in Appendix~\ref{sec:base-cv-convergence}. Since $T\bz^\star=\bz^\star$, the Cauchy--Schwarz inequality gives
\begin{align*}
\ip{\bz^+-\bz^\star}{\br}_{\bM}
&=
\ip{T\bz-T\bz^\star}{\br}_{\bM}\\
&\leq
\norm{T\bz-T\bz^\star}_{\bM}
\norm{\br}_{\bM}\\
&\leq
\norm{\bz-\bz^\star}_{\bM}
\norm{\br}_{\bM}\\
&\leq R_{\bz}e.
\end{align*}
It remains to bound $\norm{\br_{\bbeta}}_2^2$ by $e^2$. Expanding the $\bM$-norm and completing the square gives
\begin{align*}
e^2=\norm{\br}_{\bM}^2
&=
\frac1\sigma\norm{\br_{\bbeta}}_2^2
-2\ip{\bK\br_{\bbeta}}{\br_{\bnu}}
+\frac1\tau\norm{\br_{\bnu}}_2^2\\
&=
\frac1\sigma\norm{\br_{\bbeta}}_2^2
-\tau\norm{\bK\br_{\bbeta}}_2^2
+\frac1\tau\norm{\br_{\bnu}-\tau\bK\br_{\bbeta}}_2^2\\
&\geq
\frac1\sigma\norm{\br_{\bbeta}}_2^2
-\tau\norm{\bK\br_{\bbeta}}_2^2\\
&\geq
\left(\frac1\sigma-\tau\norm{\bK}_2^2\right)
\norm{\br_{\bbeta}}_2^2\\
&=
s\norm{\br_{\bbeta}}_2^2.
\end{align*}
Thus $\norm{\br_{\bbeta}}_2^2\leq e^2/s$. Combining this bound with Equation~\eqref{eq:one-step-bregman-inner-product_part_c-app} gives
\begin{equation}
B(\bzeta^+,\bu^+,\bnu^+)
\leq R_{\bz}e+\frac{L}{2s}e^2,
\end{equation}
which proves part~(c).
\end{proof}

\begin{proof}[Proof of Theorem~\ref{theorem:convergence_rate}]
Let $\{\bz^t\}_{t\geq0}$ satisfy the assumptions of the theorem, with an optimal saddle point $\bz^\star=(\bbeta^\star,\bnu^\star)$ as above, $\sigma,\tau>0$, $s=\sigma^{-1}-\tau\norm{\bK}_2^2>0$, $s\geq L_f\norm{\bA}_2^2/2$, and $\norm{\bz^t-\bz^\star}_{M}\leq R_{\bz}$ for every $t$. At each monitored point $\bz^t$, evaluate the same fixed map $T$ and its associated reconstruction $Q$:
\[
(\bbeta^{t,+},\bnu^{t,+})=T\bz^t,
\qquad
(\bzeta^{t,+},\bu^{t,+},\bnu^{t,+})=Q(\bz^t).
\]
The superscript $t,+$ denotes the output of this one-step evaluation; it need not equal the next iterate of the algorithm that generates $\{\bz^t\}$. We apply Lemma~\ref{lemma:one_step_Bregman_estimate} with $\bz=\bz^t$. Parts~(a) and~(c), together with $L=L_f\norm{\bA}_2^2$ and $e^t=\norm{(\calI-T)\bz^t}_{\bM}$, give
\begin{align}
B(\bzeta^{t,+},\bu^{t,+},\bnu^{t,+})
&\leq
R_{\bz}e^t
+\frac{L_f\norm{\bA}_2^2}{2s}(e^t)^2,
\label{eq:theorem-bregman-estimate-app}\\
\norm{V(\bzeta^{t,+},\bu^{t,+},\bnu^{t,+})}_2
&\leq
\frac{e^t}{\sqrt{\sigma}}.
\end{align}

Under Assumption~1 of the theorem, Lemma~\ref{lemma:surrogate_lower_bounds} and these two estimates yield
\begin{align*}
d^\star-\mathrm{LB}_{\mathrm{repair}}(Q(\bz^t))
&\leq
B(\bzeta^{t,+},\bu^{t,+},\bnu^{t,+})
+\bigl(L_{g^*}+\norm{\bbeta^\star}_2\bigr)
\norm{V(\bzeta^{t,+},\bu^{t,+},\bnu^{t,+})}_2\\
&\leq
R_{\bz}e^t
+\frac{L_f\norm{\bA}_2^2}{2s}(e^t)^2
+\frac{L_{g^*}+\norm{\bbeta^\star}_2}{\sqrt{\sigma}}e^t\\
&=
\left(
R_{\bz}
+\frac{L_{g^*}+\norm{\bbeta^\star}_2}{\sqrt{\sigma}}
\right)e^t
+\frac{L_f\norm{\bA}_2^2}{2s}(e^t)^2.
\end{align*}

Under Assumption~2 of the theorem, the other bound in Lemma~\ref{lemma:surrogate_lower_bounds} similarly gives
\begin{align*}
d^\star-\mathrm{LB}_{\mathrm{violation}}(Q(\bz^t))
&\leq
B(\bzeta^{t,+},\bu^{t,+},\bnu^{t,+})
+R_{\bbeta}
\norm{V(\bzeta^{t,+},\bu^{t,+},\bnu^{t,+})}_2\\
&\leq
R_{\bz}e^t
+\frac{L_f\norm{\bA}_2^2}{2s}(e^t)^2
+\frac{R_{\bbeta}}{\sqrt{\sigma}}e^t\\
&=
\left(
R_{\bz}+\frac{R_{\bbeta}}{\sqrt{\sigma}}
\right)e^t
+\frac{L_f\norm{\bA}_2^2}{2s}(e^t)^2.
\end{align*}
The nonnegativity of both lower-bound errors follows from Lemma~\ref{lemma:lower_bounds_are_valid} under the respective assumptions. These are the two inequalities stated in Theorem~\ref{theorem:convergence_rate}.
\end{proof}

The constants in these estimates may depend on the fixed node, but not on $t$. Thus, if $e^t\to0$, each applicable lower bound converges to $d^\star=p_{\calN}^\star$. More generally, if $e^t=O(\rho_t)$ for a positive sequence $\rho_t\to0$, then the corresponding lower-bound error is $O(\rho_t+\rho_t^2)=O(\rho_t)$. The theorem therefore transfers an established residual rate to the lower-bound error; it does not establish residual convergence for an arbitrary generating algorithm. For the exact fixed-step base iteration with $s>L/2$, Appendix~\ref{sec:base-cv-convergence} supplies boundedness and $e^t\to0$.
