# Supplementary material for: First-Order Primal-Dual Repairs for Scalable Branch and Bound
Source: arXiv:2610.26509 source file (2026-10-19)
Supplement: Supplementary file 5 [file D_Quadratic_loss_conj_eval.tex]

\section{Quadratic-Loss Conjugate Evaluation}
\label{app:deferred-conjugate}
\label{app:conjugate}

Both lower-bound constructions require evaluating the loss conjugate $f^*(\bzeta)$. We evaluate it at $\bzeta=\nabla f(\by)$, using the gradient already computed by the first-order method. The following identity lets us recover the conjugate value directly from $f(\by)$ and $\ip{\bzeta}{\by}$.

For a proper, closed, convex function $f$, the equality case of the Fenchel--Young inequality gives $f(\by)+f^*(\bzeta)=\ip{\bzeta}{\by}$ whenever $\bzeta\in\partial f(\by)$ \citep[Theorem~23.5]{rockafellar1970convex}. In particular, if $f$ is differentiable at $\by\in\operatorname{int}(\dom f)$ and $\bzeta:=\nabla f(\by)$, then
\begin{equation}
f^*(\bzeta)=\ip{\bzeta}{\by}-f(\by)<+\infty.
\label{eq:app-gradient}
\end{equation}

For the quadratic loss considered in the main text,
\[
f(\by)=\frac12\by^\top\bW\by-\bb^\top\by,
\qquad
\bW\in\mathbb R^{n\times n},\quad
\bW=\bW^\top\succeq0,\quad
\bb\in\mathbb R^n,
\]
the gradient is
\[
\bzeta=\nabla f(\by)=\bW\by-\bb.
\]
Substituting into Equation~\eqref{eq:app-gradient}, we obtain
\begin{align}
f^*(\bzeta)
&=\ip{\bW\by-\bb}{\by}
-\left(\frac12\by^\top\bW\by-\bb^\top\by\right)\notag\\
&=\by^\top\bW\by-\bb^\top\by
-\frac12\by^\top\bW\by+\bb^\top\by\notag\\
&=\frac12\by^\top\bW\by\notag\\
&=\frac12\ip{\by}{\bzeta+\bb}.
\label{eq:app-quadratic-conjugate}
\end{align}
The last equality uses $\bW\by=\bzeta+\bb$. Thus, once the gradient is available, the conjugate requires only a vector addition and an inner product.

In the notation of the main text, $\by^t=\bA\bbeta^t$ and $\bzeta^{t,+}=\nabla f(\by^t)$. Equation~\eqref{eq:app-quadratic-conjugate} therefore gives
\[
f^*(\bzeta^{t,+})
=\frac12\ip{\by^t}{\bzeta^{t,+}+\bb}.
\]
This evaluation requires no additional multiplication by $\bW$, linear solve, or factorization. The identity also holds when $\bW$ is singular, since the argument uses convexity and the gradient relation rather than an inverse of $\bW$.
