# Supplementary material for: First-Order Primal-Dual Repairs for Scalable Branch and Bound
Source: arXiv:2610.26509 source file (2026-10-19)
Supplement: Supplementary file 6 [file E_primal_repair.tex]

\section{Primal Repair and Early Termination}
\label{app:deferred-repair}
\label{app:primal-repair}

A lower bound supports pruning, but it does not identify when further refinement of a node relaxation cannot lead to pruning against the current incumbent. For this purpose, we also need a feasible point whose objective value bounds the node optimum from above. We construct such a point by moving the current primal iterate toward a node-compatible strictly feasible point.

We fix a node $\calN$ and retain the formulation and convexity assumptions from Appendix~\ref{app:dual-bounds}. In particular, $g$ remains the original nonsmooth objective term, $\calC_0=\calB_{\calN}$ is the zeroth block of $h$, and the sets
\[
\calC_i:=\{\bbeta\in\mathbb R^p:h_i(\bbeta)\leq0\},
\qquad i\in[m],
\]
represent the additional inequalities. The functions $h_i$ are proper, closed, and convex, so each $\calC_i$ is closed and convex. For the quantitative repair bounds below, we make the stronger endpoint and strict-slack assumptions
\begin{equation}
\bbeta^t,\ba_{\calN}\in\calB_{\calN}\cap\dom(f\circ\bA)\cap\dom g,
\qquad
h_i(\ba_{\calN})<0\quad(i\in[m]),
\label{eq:app-primal-repair-assumptions}
\end{equation}
where $\ba_{\calN}$ remains fixed for this node. The strict inequalities concern only the additional constraints; $\ba_{\calN}$ may lie on the boundary of $\calB_{\calN}$ and must respect any coordinates fixed by branching.

For $\gamma\in[0,1]$, define
\begin{equation}
\bbeta_\gamma^t:=(1-\gamma)\bbeta^t+\gamma\ba_{\calN}.
\label{eq:app-primal-segment}
\end{equation}
The choices $\gamma=0$ and $\gamma=1$ give the current iterate and the strictly feasible point, respectively. Convexity keeps the entire segment in $\calB_{\calN}\cap\dom(f\circ\bA)\cap\dom g$. This guarantees the node-box restrictions and finite loss and nonsmooth values, but not yet the additional inequalities. We choose $\gamma$ large enough to satisfy those inequalities simultaneously.

The upper-bound algorithm in the main text also includes the box as constraint block $0$. The following statement gives its certificate even when the monitored iterate lies outside that box. Its anchor need only be feasible; strict slack is required later for a quantitative displacement estimate.

\begin{proposition}[Feasibility of the full-block segment repair]
\label{prop:app-full-block-segment}
Let $\bbeta^t,\ba_{\calN}\in\dom(f\circ\bA)\cap\dom g$, and suppose $\ba_{\calN}\in\bigcap_{l=0}^m\calC_l$. For each $l=0,\ldots,m$, define
\[
\gamma_l^t:=\min\{\gamma\in[0,1]:\bbeta_\gamma^t\in\calC_l\},
\qquad
\gamma^t:=\max_{0\leq l\leq m}\gamma_l^t.
\]
Every minimum exists. The point $\bbeta_{\gamma^t}^t$ belongs to $\dom p_{\calN}$ and supplies the finite node upper bound
\[
p_{\calN}^\star\leq f(\bA\bbeta_{\gamma^t}^t)+g(\bbeta_{\gamma^t}^t)<+\infty.
\]
\end{proposition}

\begin{proof}
For each $l$, the feasible coefficient set
\[
\Gamma_l^t:=\{\gamma\in[0,1]:\bbeta_\gamma^t\in\calC_l\}
\]
is a nonempty closed interval containing $1$: the anchor belongs to $\calC_l$, and $\calC_l$ is closed and convex. Hence $\Gamma_l^t=[\gamma_l^t,1]$, with an attained minimum. Their intersection is $[\gamma^t,1]$, so $\bbeta_{\gamma^t}^t$ satisfies every constraint block, including the node box. The domains of $f\circ\bA$ and $g$ are convex and contain both endpoints; therefore the repaired point has finite values of both objective terms. It is feasible for the node relaxation, and its objective value bounds $p_{\calN}^\star$ from above.
\end{proof}

The primal proximal step in Appendix~\ref{sec:base-algorithm} produces a point in $\dom g$, but need not produce a point in $\calC_0=\calB_{\calN}$ or in the other constraint sets. When it lies outside the node box, Proposition~\ref{prop:app-full-block-segment} justifies the main-text algorithm's explicit repair of block $0$, provided both endpoints have finite objective values and the anchor is node feasible. Under the stronger condition in Equation~\eqref{eq:app-primal-repair-assumptions}, the zeroth block is satisfied along the whole segment, its exact threshold is zero, and only the additional inequalities need coefficient calculations. The displacement and convergence statements below use this stronger condition; they do not follow merely from the feasibility of the full-block repair. The dual certificates do not require primal node feasibility, and the underlying first-order updates remain unchanged.

\subsection{Feasibility and Size of the Repair}
\label{app:primal-feasibility}

\begin{proposition}[Segment repair]
\label{prop:app-segment}
Suppose that the conditions in Equation~\eqref{eq:app-primal-repair-assumptions} hold, $m\geq1$, and $h_i(\bbeta^t)$ is finite for every $i\in[m]$. Define
\begin{equation}
\gamma_i^t:=\min\{\gamma\in[0,1]:h_i(\bbeta_\gamma^t)\leq0\},
\qquad
\gamma^t:=\max_{i\in[m]}\gamma_i^t.
\label{eq:app-gamma}
\end{equation}
Algorithm~\ref{alg:compute_safe_upper_bound} writes $\alpha$ for this coefficient.
Then each minimum exists, and $\gamma^t$ is the smallest coefficient that makes the segment point satisfy all the additional inequalities. The repaired point
\begin{equation}
\bbeta_{\mathrm{rep}}^t:=\bbeta_{\gamma^t}^t
\end{equation}
belongs to $\dom p_{\calN}$ and provides the finite upper bound
\begin{equation}
p_{\calN}^\star\leq P_{\calN}^t:=f(\bA\bbeta_{\mathrm{rep}}^t)+g(\bbeta_{\mathrm{rep}}^t)<+\infty.
\label{eq:app-primal-bound}
\end{equation}

Let $s_i:=-h_i(\ba_{\calN})>0$ denote the slack at the strictly feasible point and $v_i^t:=[h_i(\bbeta^t)]_+$ the current violation, where $[z]_+:=\max\{z,0\}$. Then
\begin{equation}
0\leq\gamma_i^t\leq\widehat\gamma_i^t:=\frac{v_i^t}{v_i^t+s_i}<1.
\label{eq:app-gamma-bound}
\end{equation}
With minimum slack $\eta:=\min_{i\in[m]}s_i>0$ and maximum violation $\varepsilon^t:=\max_{i\in[m]}v_i^t$, we have
\begin{equation}
\gamma^t\leq\frac{\varepsilon^t}{\varepsilon^t+\eta},
\qquad
\norm{\bbeta_{\mathrm{rep}}^t-\bbeta^t}_2
\leq\frac{\varepsilon^t}{\varepsilon^t+\eta}\norm{\ba_{\calN}-\bbeta^t}_2.
\label{eq:app-displacement}
\end{equation}
\end{proposition}

\begin{proof}
We first show that the individual thresholds exist and that their maximum restores feasibility. For each $i\in[m]$, consider the set of feasible coefficients
\[
\Gamma_i^t:=\{\gamma\in[0,1]:\bbeta_\gamma^t\in\calC_i\}.
\]
The map $\gamma\mapsto\bbeta_\gamma^t$ is affine and continuous, and $\calC_i$ is closed and convex. Thus $\Gamma_i^t$ is a closed convex subset of $[0,1]$. It is nonempty because $\bbeta_1^t=\ba_{\calN}\in\calC_i$. Therefore, it is a compact interval containing $1$, so
\[
\Gamma_i^t=[\gamma_i^t,1].
\]
In particular, its minimum $\gamma_i^t$ is attained. A coefficient satisfies every inequality exactly when it belongs to the intersection of these intervals:
\[
\bigcap_{i=1}^m\Gamma_i^t
=\left[\max_{i\in[m]}\gamma_i^t,1\right]
=[\gamma^t,1].
\]
This proves that $\gamma^t$ is feasible for all the additional inequalities and that no smaller coefficient is feasible for all of them.

The repaired point also remains in $\calB_{\calN}\cap\dom(f\circ\bA)\cap\dom g$, because both endpoints belong to that convex set. More explicitly, convexity of the objective terms gives
\begin{align*}
f(\bA\bbeta_{\mathrm{rep}}^t)+g(\bbeta_{\mathrm{rep}}^t)
&\leq(1-\gamma^t)\bigl[f(\bA\bbeta^t)+g(\bbeta^t)\bigr]\\
&\quad+\gamma^t\bigl[f(\bA\ba_{\calN})+g(\ba_{\calN})\bigr]
<+\infty.
\end{align*}
Since the repaired point satisfies every additional inequality, $h(\bK\bbeta_{\mathrm{rep}}^t)=0$. Hence
\[
P_{\calN}^t=p_{\calN}(\bbeta_{\mathrm{rep}}^t)<+\infty,
\qquad
p_{\calN}^\star=\inf_{\bbeta}p_{\calN}(\bbeta)\leq p_{\calN}(\bbeta_{\mathrm{rep}}^t)=P_{\calN}^t,
\]
which proves Equation~\eqref{eq:app-primal-bound}.

We next derive an explicit upper bound on each threshold. For any $\gamma\in[0,1]$, convexity of $h_i$ gives
\begin{align*}
h_i(\bbeta_\gamma^t)
&\leq(1-\gamma)h_i(\bbeta^t)+\gamma h_i(\ba_{\calN})\\
&\leq(1-\gamma)v_i^t-\gamma s_i\\
&=v_i^t-\gamma(v_i^t+s_i).
\end{align*}
The denominator $v_i^t+s_i$ is strictly positive. Choosing $\gamma=\widehat\gamma_i^t:=v_i^t/(v_i^t+s_i)$ makes the final expression zero, so $\widehat\gamma_i^t\in\Gamma_i^t$. Since $\gamma_i^t$ is the minimum of $\Gamma_i^t$ and $s_i>0$,
\[
0\leq\gamma_i^t\leq\widehat\gamma_i^t=\frac{v_i^t}{v_i^t+s_i}<1.
\]
This proves Equation~\eqref{eq:app-gamma-bound}.

To obtain a bound common to all constraints, use $s_i\geq\eta$ and $v_i^t\leq\varepsilon^t$:
\[
\gamma_i^t
\leq\frac{v_i^t}{v_i^t+s_i}
\leq\frac{v_i^t}{v_i^t+\eta}
\leq\frac{\varepsilon^t}{\varepsilon^t+\eta}.
\]
The last inequality follows because $x\mapsto x/(x+\eta)$ is increasing on $[0,+\infty)$ for $\eta>0$. Taking the maximum over $i$ proves the bound on $\gamma^t$. Finally, the segment definition gives
\[
\bbeta_{\mathrm{rep}}^t-\bbeta^t=\gamma^t(\ba_{\calN}-\bbeta^t),
\]
so
\[
\norm{\bbeta_{\mathrm{rep}}^t-\bbeta^t}_2
=\gamma^t\norm{\ba_{\calN}-\bbeta^t}_2
\leq\frac{\varepsilon^t}{\varepsilon^t+\eta}\norm{\ba_{\calN}-\bbeta^t}_2.
\]
This proves Equation~\eqref{eq:app-displacement}.
\end{proof}

The exact thresholds give the smallest feasible coefficient along the chosen segment. We can also use conservative coefficients when an exact threshold is inconvenient to compute. Specifically, choose
\[
\gamma_i^t\leq\widetilde\gamma_i^t\leq\widehat\gamma_i^t,
\qquad
\widetilde\gamma^t:=\max_{i\in[m]}\widetilde\gamma_i^t.
\]
Then
\[
\gamma^t\leq\widetilde\gamma^t
\leq\max_{i\in[m]}\widehat\gamma_i^t
\leq\frac{\varepsilon^t}{\varepsilon^t+\eta}.
\]
Since $\widetilde\gamma^t\geq\gamma_i^t$ for every $i$, the point $\bbeta_{\widetilde\gamma^t}^t$ is feasible. Moreover,
\[
\norm{\bbeta_{\widetilde\gamma^t}^t-\bbeta^t}_2
=\widetilde\gamma^t\norm{\ba_{\calN}-\bbeta^t}_2
\leq\frac{\varepsilon^t}{\varepsilon^t+\eta}\norm{\ba_{\calN}-\bbeta^t}_2.
\]
Thus the conservative repair preserves feasibility, finiteness of the primal value, and the displacement bound, although it need not be minimal. The choice $\widetilde\gamma_i^t=\widehat\gamma_i^t$ is always admissible under the proposition's assumptions.

If the current iterate already satisfies all the additional inequalities, then $v_i^t=0$ for every $i$, so both the exact and conservative repairs leave it unchanged. If $m=0$ and $\bbeta^t\in\calB_{\calN}\cap\dom(f\circ\bA)\cap\dom g$, we set $\gamma^t=0$ and $\bbeta_{\mathrm{rep}}^t=\bbeta^t$ directly; no strictly feasible reference point is needed. The node-box block remains present even when there are no additional inequalities.

\subsection{Convergence of Repaired Points and Values}
\label{app:primal-convergence}

The displacement bound shows that the repair becomes small when the constraint violation becomes small, provided the distance to the strictly feasible point remains bounded. We now make this statement precise and identify the additional condition needed for convergence of the primal values.

\begin{proposition}[Vanishing repair]
\label{prop:app-primal-convergence}
Suppose that the assumptions of Proposition~\ref{prop:app-segment} hold at every monitored iteration, with the same strictly feasible point $\ba_{\calN}$. Assume that
\[
\bbeta^t\longrightarrow\overline{\bbeta}\in\dom p_{\calN},
\qquad
\varepsilon^t\longrightarrow0.
\]
Then
\[
\gamma^t\longrightarrow0,
\qquad
\bbeta_{\mathrm{rep}}^t-\bbeta^t\longrightarrow\vzero,
\qquad
\bbeta_{\mathrm{rep}}^t\longrightarrow\overline{\bbeta}.
\]
If $\overline{\bbeta}$ solves the node relaxation and $f\circ\bA+g$ is continuous at $\overline{\bbeta}$ relative to $\dom p_{\calN}$, then
\[
P_{\calN}^t\longrightarrow p_{\calN}^\star.
\]
The same conclusions hold for the conservative coefficients described above, with the primal value evaluated at the corresponding repaired point.
\end{proposition}

\begin{proof}
Since $\ba_{\calN}$ is fixed and satisfies all the inequalities strictly, its minimum slack $\eta=\min_{i\in[m]}[-h_i(\ba_{\calN})]$ is a fixed positive number. Equation~\eqref{eq:app-displacement} gives
\[
0\leq\gamma^t\leq\frac{\varepsilon^t}{\varepsilon^t+\eta}\longrightarrow0.
\]
The convergence of $\bbeta^t$ also bounds its distance to $\ba_{\calN}$, since
\[
\norm{\ba_{\calN}-\bbeta^t}_2
\leq\norm{\ba_{\calN}-\overline{\bbeta}}_2
+\norm{\bbeta^t-\overline{\bbeta}}_2.
\]
Using the segment identity, we therefore obtain
\[
\norm{\bbeta_{\mathrm{rep}}^t-\bbeta^t}_2
=\gamma^t\norm{\ba_{\calN}-\bbeta^t}_2\longrightarrow0.
\]
The triangle inequality then gives
\begin{align*}
\norm{\bbeta_{\mathrm{rep}}^t-\overline{\bbeta}}_2
&\leq\norm{\bbeta_{\mathrm{rep}}^t-\bbeta^t}_2
+\norm{\bbeta^t-\overline{\bbeta}}_2\\
&\longrightarrow0.
\end{align*}
This proves convergence of the repaired points to the same limit as the original iterates.

Each repaired point lies in $\dom p_{\calN}$. Thus, continuity of $f\circ\bA+g$ at $\overline{\bbeta}$ relative to this domain gives
\begin{align*}
P_{\calN}^t
&=(f\circ\bA+g)(\bbeta_{\mathrm{rep}}^t)\\
&\longrightarrow(f\circ\bA+g)(\overline{\bbeta})\\
&=p_{\calN}(\overline{\bbeta})
=p_{\calN}^\star.
\end{align*}
The penultimate equality uses $h(\bK\overline{\bbeta})=0$, and the last equality uses optimality of $\overline{\bbeta}$.

For a conservative repair, the same argument applies because
\[
0\leq\widetilde\gamma^t\leq\frac{\varepsilon^t}{\varepsilon^t+\eta}\longrightarrow0,
\]
and $\bbeta_{\widetilde\gamma^t}^t$ satisfies the same feasibility and displacement bounds.
\end{proof}

The assumption $\varepsilon^t\to0$ follows from iterate convergence if each $h_i$ is continuous at the limit along the iterates. Indeed, feasibility of $\overline{\bbeta}$ gives $h_i(\overline{\bbeta})\leq0$, so
\[
h_i(\bbeta^t)\longrightarrow h_i(\overline{\bbeta})\leq0
\quad\Longrightarrow\quad
v_i^t=[h_i(\bbeta^t)]_+\longrightarrow0.
\]
Since the number of inequalities is finite, $\varepsilon^t=\max_{i\in[m]}v_i^t\to0$. Affine and norm constraints satisfy this continuity condition.

We use the repaired point to evaluate $P_{\calN}^t$, while the first-order updates continue from the unrepaired iterate. Together with either finite lower bound from Appendix~\ref{app:dual-bounds}, this gives
\[
D_{\calN}^t\leq p_{\calN}^\star\leq P_{\calN}^t,
\]
where $D_{\calN}^t$ denotes the chosen lower bound. Let $U^{\mathrm{inc}}$ be the objective value of the current mixed-integer incumbent. If $D_{\calN}^t\geq U^{\mathrm{inc}}$, we can prune the node~\citep{steffy2013valid,axehill2006mixed,liang2020early}. If instead
\[
P_{\calN}^t<U^{\mathrm{inc}},
\]
then $p_{\calN}^\star\leq P_{\calN}^t<U^{\mathrm{inc}}$. Even the exact relaxation optimum is below the current pruning threshold, so further refinement of this relaxation cannot establish pruning against that incumbent. We may therefore terminate the relaxation solve and branch, provided a further integer partition is available. This conclusion concerns the current incumbent; a later improvement can change the pruning decision.

The value $P_{\calN}^t$ is an upper bound on the node relaxation, not in general on the original mixed-integer problem. We update the mixed-integer incumbent only when the repaired point also satisfies the integrality constraints and improves its value. Finally, failure to obtain a node-compatible feasible anchor makes the full-block repair unavailable; absence of strict slack prevents use of the quantitative displacement bound. Neither failure establishes that the node is infeasible.
