# Supplementary material for: First-Order Primal-Dual Repairs for Scalable Branch and Bound
Source: arXiv:2610.26509 source file (2026-10-19)
Supplement: Supplementary file 7 [file FOUR_BNB_APPENDIX_TABLES.tex]

\begin{table*}[!htbp]
\centering
\setlength{\abovecaptionskip}{0pt}
\setlength{\belowcaptionskip}{6pt}
\caption{BnB results at global relative gap $10^{-6}$.}
\label{tab:okglm-bnb-wide-1e-6}
\footnotesize
\setlength{\tabcolsep}{2pt}
\renewcommand{\arraystretch}{1.12}
\begin{tabular*}{\linewidth}{@{\extracolsep{\fill}}l*{15}{r}@{}}
\toprule
Instance & \multicolumn{3}{c}{Gurobi} & \multicolumn{3}{c}{MOSEK} & \multicolumn{3}{c}{Ours CPU} & \multicolumn{3}{c}{Ours GPU} & \multicolumn{3}{c}{Ours Batched} \\
\cmidrule(lr){2-4}\cmidrule(lr){5-7}\cmidrule(lr){8-10}\cmidrule(lr){11-13}\cmidrule(lr){14-16}
& $t$ & gap & $n$ & $t$ & gap & $n$ & $t$ & gap & $n$ & $t$ & gap & $n$ & $t$ & gap & $n$ \\
\midrule
SANTANDER & TL & -- & -- & TL & 1.69 & 3 & TL & 0.0711 & 2955 & 956.26 & 0.00 & 4767 & \textbf{71.57} & 0.00 & 6513 \\
DOROTHEA & TL & 45.58 & 1 & TL & -- & -- & 168.70 & 0.00 & 23 & 6.92 & 0.00 & 23 & \textbf{5.75} & 0.00 & 31 \\
YF-27907 & TL & -- & -- & TL & -- & -- & TL & 14.16 & 69 & 1827.24 & 0.00 & 1633 & \textbf{176.26} & 0.00 & 1633 \\
YF-35629 & TL & -- & -- & TL & 13.21 & 17 & TL & 9.30 & 266 & 2507.83 & 0.00 & 2447 & \textbf{247.74} & 0.00 & 2509 \\
squfl200-1000 & 1030.3 & 0.00 & 13.7 & 447.7 & 0.00 & 11.0 & 54.7 & 0.00 & 11.0 & 17.0 & 0.00 & 11.0 & \textbf{2.8} & 0.00 & 15.7 \\
squfl500-2500 & TL & 0.36 & 2.3 & TL & 0.01 & 5.0 & 751.9 & 0.00 & 10.3 & 30.7 & 0.00 & 10.3 & \textbf{4.2} & 0.00 & 14.3 \\
\bottomrule
\end{tabular*}
\end{table*}


\begin{table*}[!htbp]
\centering
\setlength{\abovecaptionskip}{0pt}
\setlength{\belowcaptionskip}{6pt}
\caption{Synthetic BnB results at global relative gap $10^{-4}$. TL indicates that at least one seed reached the time limit.}
\label{tab:synthetic-bnb-global-1e-4}
\scriptsize
\setlength{\tabcolsep}{1.4pt}
\renewcommand{\arraystretch}{1.0}
\begin{tabular*}{\linewidth}{@{\extracolsep{\fill}}l*{15}{r}@{}}
\toprule
Size & \multicolumn{3}{c}{Gurobi} & \multicolumn{3}{c}{MOSEK} & \multicolumn{3}{c}{ours CPU} & \multicolumn{3}{c}{ours GPU} & \multicolumn{3}{c}{ours GPU (Batched)} \\
\cmidrule(lr){2-4}\cmidrule(lr){5-7}\cmidrule(lr){8-10}\cmidrule(lr){11-13}\cmidrule(lr){14-16}
& $t$ (s) & gap (\%) & nodes & $t$ (s) & gap (\%) & nodes & $t$ (s) & gap (\%) & nodes & $t$ (s) & gap (\%) & nodes & $t$ (s) & gap (\%) & nodes \\
\midrule
\multicolumn{16}{@{}l}{\emph{Linear regression ($n=p$)}} \\
1000 & 57.0 & 0.00 & 396.3 & 30.1 & 0.00 & 21.0 & 17.4 & 0.00 & 21.0 & 5.3 & 0.00 & 21.0 & \textbf{3.2} & 0.00 & 21.0 \\
2000 & 300.2 & 0.00 & 222.7 & 143.7 & 0.00 & 21.0 & 4.1 & 0.00 & 21.0 & 3.5 & 0.00 & 21.0 & \textbf{1.8} & 0.00 & 21.0 \\
4000 & TL & 0.01 & 58.0 & 745.7 & 0.00 & 21.0 & 11.9 & 0.00 & 21.0 & 3.1 & 0.00 & 21.0 & \textbf{1.3} & 0.00 & 21.0 \\
10000 & TL & -- & -- & TL & 76.60 & 4.3 & 38.2 & 0.00 & 21.0 & 3.1 & 0.00 & 21.0 & \textbf{1.5} & 0.00 & 21.0 \\
\midrule
\multicolumn{16}{@{}l}{\emph{Logistic regression ($n=p$)}} \\
1000 & TL & 65.93 & 10514.7 & 1563.2 & 0.00 & 5553.7 & 89.1 & 0.00 & 5547.0 & 303.5 & 0.00 & 5547.7 & \textbf{8.6} & 0.00 & 6215.7 \\
2000 & TL & 64.97 & 554.0 & 1387.8 & 0.00 & 713.7 & 30.1 & 0.00 & 707.7 & 17.4 & 0.00 & 707.7 & \textbf{1.6} & 0.00 & 707.7 \\
4000 & TL & 65.97 & 1.0 & TL & 0.00 & 329.7 & 45.3 & 0.00 & 256.3 & 22.0 & 0.00 & 256.3 & \textbf{1.1} & 0.00 & 258.3 \\
10000 & TL & 72.50 & 1.0 & TL & 58.97 & 1.0 & 110.4 & 0.00 & 101.0 & 9.3 & 0.00 & 101.0 & \textbf{1.1} & 0.00 & 100.3 \\
\midrule
\multicolumn{16}{@{}l}{\emph{SQUFL ($m\times n$)}} \\
$150\times 750$ & 584.9 & 0.00 & 98.0 & 285.3 & 0.00 & 21.0 & 14.4 & 0.00 & 13.7 & 56.5 & 0.00 & 13.7 & \textbf{2.1} & 0.00 & 15.7 \\
$200\times 1000$ & 1706.0 & 0.00 & 70.0 & 401.6 & 0.00 & 8.0 & 20.4 & 0.00 & 5.7 & 10.2 & 0.00 & 5.7 & \textbf{1.3} & 0.00 & 6.3 \\
$500\times 2500$ & TL & 0.32 & 3.3 & 2729.7 & 0.00 & 3.0 & 166.4 & 0.00 & 3.7 & 13.1 & 0.00 & 3.7 & \textbf{1.5} & 0.00 & 4.3 \\
\midrule
\multicolumn{16}{@{}l}{\emph{Portfolio (k = 5)}} \\
1000 & \textbf{2.7} & 0.00 & 1.0 & 91.4 & 0.00 & 43.3 & 10.0 & 0.00 & 31.0 & 63.1 & 0.00 & 31.0 & 18.6 & 0.00 & 33.0 \\
2000 & \textbf{13.9} & 0.00 & 1.0 & 644.8 & 0.00 & 37.3 & 13.9 & 0.00 & 19.7 & 26.2 & 0.00 & 19.7 & 18.0 & 0.00 & 20.3 \\
4000 & 62.2 & 0.00 & 1.0 & TL & 0.56 & 21.3 & 116.6 & 0.00 & 59.0 & 128.1 & 0.00 & 59.0 & \textbf{27.4} & 0.00 & 59.7 \\
10000 & 1206.9 & 0.00 & 218.7 & TL & -- & -- & TL & 0.26 & 85.0 & 402.7 & 0.00 & 199.7 & \textbf{50.1} & 0.00 & 203.7 \\
\bottomrule
\end{tabular*}

\end{table*}


\begin{table*}[!htbp]
\centering
\setlength{\abovecaptionskip}{0pt}
\setlength{\belowcaptionskip}{5pt}
\caption{Synthetic BnB results at global relative gap $10^{-6}$. Unbatched regression runs already attaining $10^{-6}$ at the $10^{-4}$ target are reused, including their sample SDs.}
\label{tab:synthetic-bnb-global-1e-6}
\scriptsize
\setlength{\tabcolsep}{1.4pt}
\renewcommand{\arraystretch}{1.0}
\begin{tabular*}{\linewidth}{@{\extracolsep{\fill}}l*{15}{r}@{}}
\toprule
Size & \multicolumn{3}{c}{Gurobi} & \multicolumn{3}{c}{MOSEK} & \multicolumn{3}{c}{ours CPU} & \multicolumn{3}{c}{ours GPU} & \multicolumn{3}{c}{ours GPU (Batched)} \\
\cmidrule(lr){2-4}\cmidrule(lr){5-7}\cmidrule(lr){8-10}\cmidrule(lr){11-13}\cmidrule(lr){14-16}
& $t$ (s) & gap (\%) & nodes & $t$ (s) & gap (\%) & nodes & $t$ (s) & gap (\%) & nodes & $t$ (s) & gap (\%) & nodes & $t$ (s) & gap (\%) & nodes \\
\midrule
\multicolumn{16}{@{}l}{\emph{Linear regression ($n=p$)}} \\
1000 & 119.6 & 0.00 & 412.7 & 45.2 & 0.00 & 24.3 & 17.4 & 0.00 & 21.0 & 5.3 & 0.00 & 21.0 & \textbf{2.7} & 0.00 & 21.0 \\
2000 & 395.5 & 0.00 & 23.0 & 197.9 & 0.00 & 29.7 & 4.1 & 0.00 & 21.0 & 3.5 & 0.00 & 21.0 & \textbf{2.2} & 0.00 & 21.0 \\
4000 & 2749.5 & 0.00 & 22.7 & 1152.3 & 0.00 & 29.0 & 11.9 & 0.00 & 21.0 & 3.1 & 0.00 & 21.0 & \textbf{1.8} & 0.00 & 21.0 \\
10000 & TL & -- & -- & TL & 98.42 & 1.0 & 38.2 & 0.00 & 21.0 & \textbf{3.1} & 0.00 & 21.0 & \textbf{3.1} & 0.00 & 21.0 \\
\midrule
\multicolumn{16}{@{}l}{\emph{Logistic regression ($n=p$)}} \\
1000 & TL & 67.65 & 1941.7 & TL & 11.46 & 2001.0 & 89.1 & 0.00 & 5547.0 & 303.5 & 0.00 & 5547.7 & \textbf{15.7} & 0.00 & 5548.3 \\
2000 & TL & 67.39 & 816.3 & TL & 15.40 & 263.7 & 30.1 & 0.00 & 707.7 & 17.4 & 0.00 & 707.7 & \textbf{2.5} & 0.00 & 707.7 \\
4000 & TL & 90.72 & 1.0 & TL & 16.00 & 35.0 & 45.3 & 0.00 & 256.3 & 22.0 & 0.00 & 256.3 & \textbf{2.0} & 0.00 & 256.3 \\
10000 & TL & -- & -- & TL & -- & -- & 110.4 & 0.00 & 101.0 & 9.3 & 0.00 & 101.0 & \textbf{2.0} & 0.00 & 101.0 \\
\midrule
\multicolumn{16}{@{}l}{\emph{SQUFL ($m\times n$)}} \\
$150\times 750$ & 798.9 & 0.00 & 21.0 & 429.5 & 0.00 & 21.0 & 34.9 & 0.00 & 18.3 & 26.3 & 0.00 & 18.3 & \textbf{2.9} & 0.00 & 17.7 \\
$200\times 1000$ & 1030.3 & 0.00 & 13.7 & 447.7 & 0.00 & 11.0 & 54.7 & 0.00 & 11.0 & 17.0 & 0.00 & 11.0 & \textbf{2.8} & 0.00 & 15.7 \\
$500\times 2500$ & TL & 0.36 & 2.3 & TL & 0.01 & 5.0 & 751.9 & 0.00 & 10.3 & 30.7 & 0.00 & 10.3 & \textbf{4.2} & 0.00 & 14.3 \\
\midrule
\multicolumn{16}{@{}l}{\emph{Portfolio ($k=5$)}} \\
1000 & \textbf{5.0} & 0.00 & 50.3 & 141.3 & 0.00 & 46.3 & 14.9 & 0.00 & 33.0 & 30.6 & 0.00 & 33.0 & 19.7 & 0.00 & 33.0 \\
2000 & 36.1 & 0.00 & 19.3 & 896.8 & 0.00 & 37.7 & 42.0 & 0.00 & 24.3 & 34.3 & 0.00 & 24.3 & \textbf{27.6} & 0.00 & 24.3 \\
4000 & 166.6 & 0.00 & 114.7 & TL & 1.45 & 9.0 & 169.4 & 0.00 & 60.3 & 78.2 & 0.00 & 60.3 & \textbf{30.0} & 0.00 & 60.3 \\
10000 & TL & 0.01 & 262.7 & TL & -- & -- & TL & 0.39 & 55.7 & 325.7 & 0.00 & 203.7 & \textbf{50.2} & 0.00 & 203.7 \\
\bottomrule
\end{tabular*}
\end{table*}

\clearpage
\begin{table*}[!htbp]
\centering
\setlength{\abovecaptionskip}{0pt}
\setlength{\belowcaptionskip}{5pt}
\caption{Synthetic BnB sample standard deviations at global relative gap $10^{-4}$: solver time $s_t$ (s) and nodes $s_N$.}
\label{tab:synthetic-bnb-sd-1e-4}
\footnotesize
\setlength{\tabcolsep}{3pt}
\renewcommand{\arraystretch}{1.0}
\begin{tabular*}{\linewidth}{@{\extracolsep{\fill}}l*{10}{r}@{}}
\toprule
Size & \multicolumn{2}{c}{Gurobi} & \multicolumn{2}{c}{MOSEK} & \multicolumn{2}{c}{Ours CPU} & \multicolumn{2}{c}{Ours GPU} & \multicolumn{2}{c}{Ours Batched} \\
\cmidrule(lr){2-3}\cmidrule(lr){4-5}\cmidrule(lr){6-7}\cmidrule(lr){8-9}\cmidrule(lr){10-11}
& $s_t$ & $s_N$ & $s_t$ & $s_N$ & $s_t$ & $s_N$ & $s_t$ & $s_N$ & $s_t$ & $s_N$ \\
\midrule
\multicolumn{11}{@{}l}{\emph{Linear regression ($n=p$)}} \\
1000 & 28.6 & 326.4 & 1.3 & 0 & 0.36 & 0 & 2.8 & 0 & 1.2 & 0 \\
2000 & 27.2 & 41.5 & 3.7 & 0 & 0.60 & 0 & 2.8 & 0 & 0.17 & 0 \\
4000 & 1039.2 & 31.2 & 26.6 & 0 & 1.1 & 0 & 1.3 & 0 & 0.11 & 0 \\
10000 & 19.9 & 0 & 7.5 & 1.5 & 3.6 & 0 & 1.3 & 0 & 0.26 & 0 \\
\midrule
\multicolumn{11}{@{}l}{\emph{Logistic regression ($n=p$)}} \\
1000 & 0.48 & 1598.1 & 925.9 & 3526.1 & 49.3 & 3467.5 & 81.7 & 3466.8 & 4.0 & 3901.8 \\
2000 & 0.35 & 56.9 & 292.5 & 177.5 & 7.6 & 186.0 & 3.6 & 186.0 & 0.20 & 183.0 \\
4000 & 0.42 & 0 & 207.4 & 35.6 & 4.8 & 32.6 & 13.5 & 32.6 & 0.05 & 32.6 \\
10000 & 7.0 & 0 & 4.2 & 0 & 19.6 & 20.8 & 4.6 & 20.8 & 0.01 & 19.6 \\
\midrule
\multicolumn{11}{@{}l}{\emph{SQUFL ($m\times n$)}} \\
$150\times 750$ & 351.2 & 72.6 & 92.5 & 15.7 & 4.1 & 6.1 & 39.9 & 6.1 & 0.59 & 7.6 \\
$200\times 1000$ & 564.2 & 41.2 & 123.7 & 4.6 & 9.9 & 3.1 & 5.3 & 3.1 & 0.26 & 3.1 \\
$500\times 2500$ & 5.3 & 1.2 & 297.2 & 2.8 & 35.9 & 1.2 & 3.1 & 1.2 & 0.25 & 1.2 \\
\midrule
\multicolumn{11}{@{}l}{\emph{Portfolio ($k=5$)}} \\
1000 & 0.38 & 0 & 35.3 & 32.6 & 4.8 & 19.7 & 14.5 & 19.7 & 4.6 & 21.6 \\
2000 & 0.66 & 0 & 170.2 & 22.7 & 6.7 & 12.2 & 12.9 & 12.2 & 5.7 & 11.4 \\
4000 & 5.2 & 0 & 186.0 & 8.4 & 129.3 & 71.2 & 106.9 & 71.2 & 9.6 & 72.3 \\
10000 & 432.0 & 377.0 & 33.8 & 0 & 1776.4 & 85.8 & 378.4 & 281.3 & 21.5 & 286.6 \\
\bottomrule
\end{tabular*}
\end{table*}

\begin{table*}[!htbp]
\centering
\setlength{\abovecaptionskip}{0pt}
\setlength{\belowcaptionskip}{5pt}
\caption{Synthetic BnB sample standard deviations at global relative gap $10^{-6}$: solver time $s_t$ (s) and nodes $s_N$.}
\label{tab:synthetic-bnb-sd-1e-6}
\footnotesize
\setlength{\tabcolsep}{3pt}
\renewcommand{\arraystretch}{1.0}
\begin{tabular*}{\linewidth}{@{\extracolsep{\fill}}l*{10}{r}@{}}
\toprule
Size & \multicolumn{2}{c}{Gurobi} & \multicolumn{2}{c}{MOSEK} & \multicolumn{2}{c}{Ours CPU} & \multicolumn{2}{c}{Ours GPU} & \multicolumn{2}{c}{Ours Batched} \\
\cmidrule(lr){2-3}\cmidrule(lr){4-5}\cmidrule(lr){6-7}\cmidrule(lr){8-9}\cmidrule(lr){10-11}
& $s_t$ & $s_N$ & $s_t$ & $s_N$ & $s_t$ & $s_N$ & $s_t$ & $s_N$ & $s_t$ & $s_N$ \\
\midrule
\multicolumn{11}{@{}l}{\emph{Linear regression ($n=p$)}} \\
1000 & 75.8 & 399.7 & 5.4 & 5.8 & 0.36 & 0 & 2.8 & 0 & 0.23 & 0 \\
2000 & 29.3 & 0 & 1.2 & 1.2 & 0.60 & 0 & 2.8 & 0 & 0.09 & 0 \\
4000 & 340.0 & 0.58 & 38.5 & 0 & 1.1 & 0 & 1.3 & 0 & 0.12 & 0 \\
10000 & 0.16 & 0 & 6.3 & 0 & 3.6 & 0 & 1.3 & 0 & 1.3 & 0 \\
\midrule
\multicolumn{11}{@{}l}{\emph{Logistic regression ($n=p$)}} \\
1000 & 0.67 & 190.0 & 0.25 & 97.6 & 49.3 & 3467.5 & 81.7 & 3466.8 & 9.6 & 3467.9 \\
2000 & 0.15 & 447.0 & 0.24 & 44.5 & 7.6 & 186.0 & 3.6 & 186.0 & 0.30 & 186.0 \\
4000 & 0.30 & 0 & 6.5 & 10.4 & 4.8 & 32.6 & 13.5 & 32.6 & 0.17 & 32.6 \\
10000 & 0.34 & 0 & 49.0 & 0 & 19.6 & 20.8 & 4.6 & 20.8 & 0.09 & 20.8 \\
\midrule
\multicolumn{11}{@{}l}{\emph{SQUFL ($m\times n$)}} \\
$150\times 750$ & 297.0 & 8.7 & 185.6 & 14.0 & 16.0 & 9.9 & 11.5 & 9.9 & 0.73 & 9.2 \\
$200\times 1000$ & 360.1 & 5.8 & 140.4 & 4.0 & 9.1 & 2.0 & 3.6 & 2.0 & 1.5 & 8.3 \\
$500\times 2500$ & 4.1 & 0.58 & 396.4 & 2.0 & 368.0 & 4.6 & 10.9 & 4.6 & 2.1 & 10.1 \\
\midrule
\multicolumn{11}{@{}l}{\emph{Portfolio ($k=5$)}} \\
1000 & 2.5 & 24.9 & 83.5 & 33.1 & 13.5 & 21.6 & 16.3 & 21.6 & 5.5 & 21.6 \\
2000 & 9.9 & 6.4 & 321.0 & 21.9 & 32.3 & 14.5 & 17.1 & 14.5 & 10.1 & 14.5 \\
4000 & 15.7 & 117.2 & 1.3 & 3.5 & 171.8 & 73.5 & 80.1 & 73.5 & 9.3 & 73.5 \\
10000 & 763.5 & 332.3 & 60.7 & 0 & 1644.4 & 40.2 & 420.3 & 286.6 & 17.6 & 286.6 \\
\bottomrule
\end{tabular*}
\end{table*}
