# Supplementary material for: First-Order Primal-Dual Repairs for Scalable Branch and Bound
Source: arXiv:2610.26509 source file (2026-10-19)
Supplement: Supplementary file 8 [file F_anchor.tex]

\section{Computing the Anchor and the Repair}
\label{app:repair-formulas}

Appendix~\ref{app:primal-repair} constructs a feasible point by moving the current iterate toward a node-compatible strictly feasible point. We now describe how to find this anchor and compute the segment coefficients for the constraint families considered here. We retain the notation $h_i$, $\ba_{\calN}$, $s_i$, and $v_i^t$ from that appendix and distinguish exact thresholds from conservative coefficients.

\subsection{Node-Compatible Anchors}
\label{app:anchors}

The node box is the zeroth constraint block $\calC_0=\calB_{\calN}$ in the splitting used throughout the appendix. The anchor must satisfy the restrictions of the current node, including any coordinates fixed by branching, and have finite objective value. It must also satisfy strictly every inequality for which we use a positive-slack repair. We may reuse a parent anchor only after checking that it still meets these conditions at the child node.

To search for an anchor when $m\geq1$, choose a nonempty convex set
\[
\calS_{\calN}\subseteq\calB_{\calN}\cap\dom(f\circ\bA)\cap\dom g
\]
and consider the supremum of the minimum constraint slack:
\begin{equation}
\rho^\star:=\sup_{\bv\in\calS_{\calN}}\min_{i\in[m]}\{-h_i(\bv)\}
=-\inf_{\bv\in\calS_{\calN}}\max_{i\in[m]}h_i(\bv).
\label{eq:app-anchor-margin}
\end{equation}
The second expression minimizes a convex function, since the pointwise maximum of finitely many convex functions is convex. Equivalently, we can introduce an explicit slack variable and write
\begin{equation}
\begin{aligned}
\rho^\star=\sup_{\bv,\rho}\quad &\rho\\
\text{subject to}\quad &\bv\in\calS_{\calN},\qquad \rho\in\mathbb R,\\
&h_i(\bv)+\rho\leq0,\qquad i\in[m].
\end{aligned}
\label{eq:app-anchor-phase-one}
\end{equation}
For any feasible pair $(\bv,\rho)$ with $\rho>0$, every inequality satisfies $h_i(\bv)\leq-\rho<0$. Thus $\ba_{\calN}:=\bv$ is a valid anchor. We do not need to attain $\rho^\star$: any returned point $\ba_{\calN}\in\calS_{\calN}$ with
\[
\eta:=\min_{i\in[m]}\{-h_i(\ba_{\calN})\}>0
\]
is sufficient for the repair in Proposition~\ref{prop:app-segment}. For affine inequalities, Equation~\eqref{eq:app-anchor-phase-one} is a max-margin Phase-I formulation. Failure to find a positive-slack point within the allotted budget does not establish node infeasibility.

Some constraints require no repair because both segment endpoints already satisfy them. If $h_i(\bbeta^t)\leq0$ and $h_i(\ba_{\calN})\leq0$, then convexity gives
\[
h_i(\bbeta_\gamma^t)
\leq(1-\gamma)h_i(\bbeta^t)+\gamma h_i(\ba_{\calN})
\leq0
\qquad\text{for every }\gamma\in[0,1].
\]
Its feasible coefficient interval is therefore $[0,1]$, and its exact threshold is zero. We can omit such an inequality from the coefficient calculation, even when its slack at the anchor is zero. We apply Proposition~\ref{prop:app-segment} to the remaining inequalities, which must have strictly positive anchor slacks, and take the minimum slack and maximum violation over that collection. The anchor search can likewise omit inequalities that the search set and every monitored iterate already satisfy. If no inequalities remain, we use the identity repair from Appendix~\ref{app:primal-repair}.

Affine equalities are preserved in the same way. Let $\bE\in\mathbb R^{q\times p}$ and $\bb_{\mathrm{eq}}\in\mathbb R^q$ describe retained equalities, and suppose
\[
\bE\bbeta^t=\bE\ba_{\calN}=\bb_{\mathrm{eq}}.
\]
Then
\begin{equation}
\bE\bbeta_\gamma^t
=(1-\gamma)\bE\bbeta^t+\gamma\bE\ba_{\calN}
=(1-\gamma)\bb_{\mathrm{eq}}+\gamma\bb_{\mathrm{eq}}
=\bb_{\mathrm{eq}}.
\label{eq:app-retained-equalities}
\end{equation}
In particular, coordinates fixed by branching remain fixed along the segment. These equalities require no strict slack when both endpoints satisfy them.

\subsection{Constraint Functions and Repair Coefficients}
\label{app:parallel-repair}

For each inequality requiring a positive-slack repair, we cache
\[
s_i:=-h_i(\ba_{\calN})>0
\]
while the anchor and that constraint remain unchanged. At iteration $t$, we compute
\[
v_i^t:=[h_i(\bbeta^t)]_+.
\]
The exact threshold $\gamma_i^t$ is the smallest feasible coefficient along the segment. The conservative coefficient from Appendix~\ref{app:primal-repair} is
\[
\widehat\gamma_i^t:=\frac{v_i^t}{v_i^t+s_i}.
\]
Both coefficients are zero when $v_i^t=0$. Table~\ref{tab:app-repair-coefficients} gives formulas for violated inequalities, where $v_i^t>0$. We use the exact threshold for affine inequalities and Euclidean balls, and the conservative coefficient for the $\ell_1$-ball and second-order cone rows.

For Euclidean balls, cache the displacement of the anchor from each center,
\[
\be_i:=\ba_{\calN}-\bc_i,
\]
and compute
\begin{equation}
\Delta\bbeta^t:=\bbeta^t-\ba_{\calN},
\qquad
\kappa^t:=\norm{\Delta\bbeta^t}_2^2,
\qquad
\omega_i^t:=\ip{\be_i}{\Delta\bbeta^t}.
\label{eq:app-ball-quantities}
\end{equation}
The direction $\Delta\bbeta^t$ and its squared norm $\kappa^t$ are shared across all balls in the same decision space.

In the affine row, $\bc_i\in\mathbb R^p$ and $b_i\in\mathbb R$ specify the halfspace. In the ball rows, $\bc_i$ denotes the center and $R_i>0$ the radius. The constants $L_j,U_j$ are finite coordinate bounds, and $a_{\calN,j}:=(\ba_{\calN})_j$ is the corresponding scalar anchor component. In the second-order cone row, $\bx_i$ and $\theta_i$ are fixed affine maps with vector and scalar outputs, respectively. In the SQUFL row, $\ell$ indexes facilities and $j$ indexes customers; $\beta_{\ell j}$ and $a_{\calN,\ell j}$ denote the scalar allocation components of the iterate and anchor.

\begin{table*}[t]
\centering
\small
\setlength{\tabcolsep}{4pt}
\renewcommand{\arraystretch}{1.8}
\caption{Constraint functions, cached anchor slacks, and segment coefficients for violated inequalities with strictly positive anchor slack. The affine and Euclidean-ball formulas give exact thresholds $\gamma_i^t$; the $\ell_1$-ball and second-order cone formulas give conservative coefficients $\widehat\gamma_i^t$. Every coefficient is zero when the current point satisfies the corresponding inequality.}
\vspace{2mm}
\label{tab:app-repair-coefficients}
\begin{tabular}{@{}llll@{}}
\toprule
Constraint & $h_i(\bbeta)$ & Cached slack $s_i=-h_i(\ba_{\calN})$ & Repair coefficient \\
\midrule
Affine inequality & $\bc_i^\top\bbeta-b_i$ & $b_i-\bc_i^\top\ba_{\calN}$ & $\displaystyle\gamma_i^t=\frac{v_i^t}{v_i^t+s_i}$ \\
Coordinate lower bound & $L_j-\beta_j$ & $a_{\calN,j}-L_j$ & $\displaystyle\gamma_i^t=\frac{v_i^t}{v_i^t+s_i}$ \\
Coordinate upper bound & $\beta_j-U_j$ & $U_j-a_{\calN,j}$ & $\displaystyle\gamma_i^t=\frac{v_i^t}{v_i^t+s_i}$ \\
$\ell_2$-ball & $\norm{\bbeta-\bc_i}_2^2-R_i^2$ & $R_i^2-\norm{\ba_{\calN}-\bc_i}_2^2$ & $\displaystyle\gamma_i^t=1-\frac{\sqrt{(\omega_i^t)^2+\kappa^t s_i}-\omega_i^t}{\kappa^t}$ \\
$\ell_1$-ball & $\norm{\bbeta-\bc_i}_1-R_i$ & $R_i-\norm{\ba_{\calN}-\bc_i}_1$ & $\displaystyle\widehat\gamma_i^t=\frac{v_i^t}{v_i^t+s_i}$ \\
Second-order cone & $\norm{\bx_i(\bbeta)}_2-\theta_i(\bbeta)$ & $\theta_i(\ba_{\calN})-\norm{\bx_i(\ba_{\calN})}_2$ & $\displaystyle\widehat\gamma_i^t=\frac{v_i^t}{v_i^t+s_i}$ \\
SQUFL coverage & $\displaystyle h_j(\bbeta)=1-\sum_\ell\beta_{\ell j}$ & $\displaystyle s_j=\sum_\ell a_{\calN,\ell j}-1$ & $\displaystyle\gamma_j^t=\frac{v_j^t}{v_j^t+s_j}$ \\
\bottomrule
\end{tabular}
\end{table*}

The coordinate-bound rows are included for completeness. Under the stronger endpoint-feasibility assumption in Appendix~\ref{app:primal-repair}, bounds defining $\calB_{\calN}$ hold at both segment endpoints and need no repair. The full-block repair of Proposition~\ref{prop:app-full-block-segment} also applies when the monitored point violates a box bound. For a finite lower or upper coordinate bound, let $v>0$ be its violation and $s\geq0$ its slack at the feasible anchor. Since the constraint is affine, its exact threshold is $v/(v+s)$, including the case $s=0$, for which the threshold is $1$. A satisfied coordinate bound has threshold $0$. Taking the maximum over finite coordinate bounds gives the threshold for block $0$; an absent infinite bound contributes no constraint. Thus a coordinate fixed by branching requires no strict anchor slack, although an iterate that violates that fixed coordinate may have to move all the way to the anchor. In this zero-slack case the displacement estimate of Proposition~\ref{prop:app-segment} does not apply. The Euclidean-ball row uses the squared-norm constraint, so its violation and cached slack must both use that same representation.

\paragraph{Affine inequalities.}
For $h_i(\bbeta)=\bc_i^\top\bbeta-b_i$, affinity gives
\begin{align*}
h_i(\bbeta_\gamma^t)
&=\bc_i^\top\bigl((1-\gamma)\bbeta^t+\gamma\ba_{\calN}\bigr)-b_i\\
&=(1-\gamma)\bigl(\bc_i^\top\bbeta^t-b_i\bigr)+\gamma\bigl(\bc_i^\top\ba_{\calN}-b_i\bigr)\\
&=(1-\gamma)h_i(\bbeta^t)-\gamma s_i.
\end{align*}
If the current point violates this inequality, then $h_i(\bbeta^t)=v_i^t>0$, and
\[
h_i(\bbeta_\gamma^t)\leq0
\quad\Longleftrightarrow\quad
v_i^t-\gamma(v_i^t+s_i)\leq0
\quad\Longleftrightarrow\quad
\gamma\geq\frac{v_i^t}{v_i^t+s_i}.
\]
If the current point is feasible, the smallest coefficient is zero. Both cases therefore give
\begin{equation}
\gamma_i^t=\frac{v_i^t}{v_i^t+s_i}.
\label{eq:app-affine-gamma}
\end{equation}
For affine inequalities, the convexity bound from Appendix~\ref{app:primal-repair} is thus exact. Coordinate bounds, SQUFL coverage, regression links, selector budgets, and the affine portfolio inequalities all use this formula.

For example, the SQUFL coverage inequality for customer $j$ has
\[
h_j(\bbeta)=1-\sum_\ell\beta_{\ell j},
\qquad
s_j=\sum_\ell a_{\calN,\ell j}-1>0,
\qquad
v_j^t=\left[1-\sum_\ell\beta_{\ell j}^t\right]_+.
\]
Along the segment,
\[
1-\sum_\ell(\bbeta_\gamma^t)_{\ell j}
=(1-\gamma)\left(1-\sum_\ell\beta_{\ell j}^t\right)-\gamma s_j,
\]
so its exact threshold is $\gamma_j^t=v_j^t/(v_j^t+s_j)$.

\paragraph{Euclidean balls.}
Consider $h_i(\bbeta)=\norm{\bbeta-\bc_i}_2^2-R_i^2$. Since $\ba_{\calN}$ lies strictly inside the ball, its cached slack is
\[
s_i=R_i^2-\norm{\be_i}_2^2>0.
\]
Set $\alpha:=1-\gamma$. Using Equation~\eqref{eq:app-ball-quantities}, we can write the segment point relative to the center as
\[
\bbeta_\gamma^t-\bc_i
=\ba_{\calN}-\bc_i+\alpha(\bbeta^t-\ba_{\calN})
=\be_i+\alpha\Delta\bbeta^t.
\]
Expanding the squared norm gives
\begin{align*}
h_i(\bbeta_\gamma^t)
&=\norm{\be_i+\alpha\Delta\bbeta^t}_2^2-R_i^2\\
&=\norm{\be_i}_2^2+2\alpha\ip{\be_i}{\Delta\bbeta^t}+\alpha^2\norm{\Delta\bbeta^t}_2^2-R_i^2\\
&=\kappa^t\alpha^2+2\omega_i^t\alpha-s_i.
\end{align*}
Thus feasibility is equivalent to
\begin{equation}
\kappa^t\alpha^2+2\omega_i^t\alpha-s_i\leq0,
\qquad \alpha\in[0,1].
\label{eq:app-ball-quadratic}
\end{equation}
For a violated ball, $\kappa^t>0$: otherwise $\bbeta^t=\ba_{\calN}$, contradicting strict feasibility of the anchor. The quadratic in Equation~\eqref{eq:app-ball-quadratic} is negative at $\alpha=0$ and positive at $\alpha=1$. Moreover, the product of its roots is $-s_i/\kappa^t<0$, so it has exactly one positive root. This root is
\[
\alpha_i^t=\frac{\sqrt{(\omega_i^t)^2+\kappa^t s_i}-\omega_i^t}{\kappa^t}\in(0,1).
\]
Within $[0,1]$, the feasible values are exactly $\alpha\in[0,\alpha_i^t]$. Since $\gamma=1-\alpha$, the smallest feasible repair coefficient is
\begin{equation}
\gamma_i^t
=1-\alpha_i^t
=1-\frac{\sqrt{(\omega_i^t)^2+\kappa^t s_i}-\omega_i^t}{\kappa^t}.
\label{eq:app-ball-gamma}
\end{equation}
When the current point is already in the ball, we set $\gamma_i^t=0$ without evaluating the root formula. In particular, this avoids division by zero when $\bbeta^t=\ba_{\calN}$.

\paragraph{$\ell_1$ balls and second-order cones.}
For these rows, we use the conservative coefficient rather than compute an exact threshold. The $\ell_1$-ball constraint is convex because it is a norm of an affine expression minus a constant. The second-order cone constraint is also convex: $\bx_i$ and $\theta_i$ are affine, and the Euclidean norm is convex. More explicitly,
\begin{align*}
\norm{\bx_i(\bbeta_\gamma^t)}_2
&=\norm{(1-\gamma)\bx_i(\bbeta^t)+\gamma\bx_i(\ba_{\calN})}_2\\
&\leq(1-\gamma)\norm{\bx_i(\bbeta^t)}_2+\gamma\norm{\bx_i(\ba_{\calN})}_2,
\end{align*}
while
\[
\theta_i(\bbeta_\gamma^t)
=(1-\gamma)\theta_i(\bbeta^t)+\gamma\theta_i(\ba_{\calN}).
\]
Subtracting the scalar affine expression gives the convexity bound for the cone constraint. The $\ell_1$-ball constraint satisfies the same bound by convexity of the $\ell_1$ norm. In either case,
\begin{align*}
h_i(\bbeta_\gamma^t)
&\leq(1-\gamma)h_i(\bbeta^t)+\gamma h_i(\ba_{\calN})\\
&\leq(1-\gamma)v_i^t-\gamma s_i\\
&=v_i^t-\gamma(v_i^t+s_i).
\end{align*}
Choosing $\gamma=\widehat\gamma_i^t=v_i^t/(v_i^t+s_i)$ makes the right-hand side zero. Hence the coefficient is feasible, although it need not be the smallest feasible one. This is exactly the conservative construction in Equation~\eqref{eq:app-gamma-bound}.

\paragraph{Parallel evaluation.}
The cached slacks depend only on the anchor and the constraint parameters. At a monitored iteration, we evaluate the constraint values and compute their coefficients independently. Let $\widetilde\gamma_i^t$ denote the returned coefficient: the exact $\gamma_i^t$ for an affine or Euclidean-ball constraint, the conservative $\widehat\gamma_i^t$ for an $\ell_1$-ball or cone constraint, and zero for an inequality satisfied at both endpoints. A maximum reduction gives
\[
\widetilde\gamma^t:=\max_i\widetilde\gamma_i^t.
\]
For every inequality requiring repair, $\widetilde\gamma_i^t\geq\gamma_i^t$, so $\widetilde\gamma^t$ belongs to its feasible interval $[\gamma_i^t,1]$. The inequalities omitted from the calculation hold along the whole segment. Therefore,
\[
\bbeta_{\widetilde\gamma^t}^t
=(1-\widetilde\gamma^t)\bbeta^t+\widetilde\gamma^t\ba_{\calN}
\]
is feasible and satisfies the conservative-repair displacement bound from Appendix~\ref{app:primal-repair}. When every returned coefficient is exact, $\widetilde\gamma^t=\gamma^t$; otherwise the common coefficient can be larger than the minimum.

For a collection of affine inequalities, write $\bm{C}\bbeta\leq\bb_{\mathrm{aff}}$, where $\bm{C}$ contains their row vectors; this matrix is distinct from the loss matrix $\bA$. We cache
\[
\bs:=\bb_{\mathrm{aff}}-\bm{C}\ba_{\calN}
\]
and compute $\bm{C}\bbeta^t-\bb_{\mathrm{aff}}$ at the current iterate. On rows with strictly positive cached slack, positive parts and elementwise ratios give
\[
v_i^t=[(\bm{C}\bbeta^t-\bb_{\mathrm{aff}})_i]_+,
\qquad
\gamma_i^t=\frac{v_i^t}{v_i^t+s_i}.
\]
Norm constraints similarly use independent norms or inner products. For Euclidean balls, the direction and squared norm in Equation~\eqref{eq:app-ball-quantities} are computed once and reused across centers. The final segment update is elementwise. Once the anchor is available, these coefficient evaluations and the segment update require no linear solve; the anchor search is a separate computation.
