# Supplementary material for: First-Order Primal-Dual Repairs for Scalable Branch and Bound
Source: arXiv:2610.26509 source file (2026-10-19)
Supplement: Supplementary file 9 [file G_problems_and_data.tex]

\section{Problem Classes and Experimental Setup}
\label{app:experimental-setup}

We study sparse linear and logistic regression, separable quadratic uncapacitated facility location (SQUFL), and sparse portfolio optimization on synthetic instances of increasing size. The real-data benchmarks are DOROTHEA~\citep{guyon2004result} for classification, SANTANDER~\citep{santander} for regression, and two fixed Yahoo Finance return datasets for portfolio optimization. Our SQUFL instances are synthetic and follow the quadratic facility-location structure represented in MINLPLib~\citep{bussieck2003minlplib}; they are not downloaded MINLPLib instances. Below we specify the models, data construction, and computational protocol. Further results appear in Appendix~\ref{app:additional-experiments}; the primal repair and its constraint-specific coefficients are developed in Appendices~\ref{app:primal-repair} and~\ref{app:repair-formulas}. In all four problem classes, segment repair handles affine constraints: the rows $\bm{C}\bbeta\leq\bb_{\mathrm{aff}}$, the SQUFL covering inequalities, and the portfolio budget and return floor. Cardinality, selector bounds, and perspective terms are handled by the proximable term $g_{\calN}$ (Appendix~\ref{app:computational-protocol}). Proposition~\ref{prop:app-full-block-segment} requires a feasible anchor, whereas Proposition~\ref{prop:app-segment} additionally assumes strict slack for its quantitative bounds; Appendix~\ref{app:parallel-repair} gives repair coefficients for Euclidean balls, $\ell_1$-balls, and second-order cones.

\subsection{Problem Formulations}
\label{app:problem-formulations}

We define the variables and dimensions separately for each problem class. We use $\bm{C}$ for matrices of additional linear constraints, distinguishing them from the loss matrix $\bA$ in the general formulation. In regression, $\bX$ denotes the data matrix, and $f(\bX\bbeta)$ is the corresponding smooth loss.

\paragraph{Sparse linear and logistic regression.}
We consider models with at most $k$ nonzero coefficients, bounded coefficient magnitudes, and additional linear inequalities:
\begin{equation}
\begin{aligned}
\min_{\bbeta,\bz}\quad
    & f(\bX\bbeta)+\lambda_2\norm{\bbeta}_2^2\\
\mathrm{s.t.}\quad
    & |\beta_j|\leq Mz_j,\qquad j\in[p],\\
    & \vone^\top\bz\leq k,\qquad \bz\in\{0,1\}^p,\\
    & \bm{C}\bbeta\leq\bb_{\mathrm{aff}}.
\end{aligned}
\label{eq:exp-regression}
\end{equation}
Here, $\bX\in\mathbb R^{n\times p}$ contains $n$ observations and $p$ features, and $\bbeta\in\mathbb R^p$ is the coefficient vector. The function $f$ is the squared loss for regression or the logistic loss for classification, and $\lambda_2$ controls ridge regularization. The binary variable $z_j$ indicates whether feature $j$ is selected, while $M$ bounds the magnitude of a selected coefficient. In all reported regression experiments we set $k=10$ and $\lambda_2=1$; we use $M=2$ for synthetic instances and $M=10$ for real-data instances. Each instance has ten additional affine inequalities, so $\bm{C}\in\mathbb R^{10\times p}$ and $\bb_{\mathrm{aff}}\in\mathbb R^{10}$. These ten rows are in addition to the cardinality inequality and the $2p$ scalar linear inequalities represented by $|\beta_j|\leq Mz_j$.

\paragraph{Separable quadratic uncapacitated facility location.}
We allocate customer demand among selected facilities, with fixed opening costs and quadratic allocation costs:
\begin{equation}
\begin{aligned}
\min_{\bbeta,\bz}\quad
    & \sum_{i=1}^{m}c_i z_i+\sum_{i=1}^{m}\sum_{j=1}^{n}q_{ij}\beta_{ij}^2\\
\mathrm{s.t.}\quad
    & \sum_{i=1}^{m}\beta_{ij}=1,\qquad j\in[n],\\
    & 0\leq\beta_{ij}\leq z_i,\qquad i\in[m],\ j\in[n],\\
    & \bz\in\{0,1\}^{m}.
\end{aligned}
\label{eq:exp-facility}
\end{equation}
Here, $m$ and $n$ denote the numbers of facilities and customers. The binary variable $z_i$ indicates whether facility $i$ is open, and $\beta_{ij}$ is the fraction of customer $j$'s demand assigned to facility $i$. The coefficients $c_i$ and $q_{ij}\geq0$ specify the opening and quadratic allocation costs, respectively.

For the node relaxations, we replace the assignment equalities with the covering inequalities
\[
\sum_{i=1}^{m}\beta_{ij}\geq1,\qquad j\in[n].
\]
This replacement preserves the optimal value. Any excess allocation can be reduced to satisfy the assignment equalities while preserving $0\leq\beta_{ij}\leq z_i$. Since $q_{ij}\geq0$, this reduction cannot increase the objective. Conversely, every point satisfying the assignment equalities satisfies the covering inequalities. With $q_{ij}>0$, reducing excess allocation strictly lowers the objective, so the covering inequalities are active at every feasible node optimum. The repair coefficient for SQUFL coverage is given in Appendix~\ref{app:parallel-repair}.

\paragraph{Sparse portfolio optimization.}
For the synthetic instances, we use the sparse ridge-regularized mean--variance model of \citet{bertsimas2022scalable}:
\begin{equation}
\begin{aligned}
\min_{\bbeta\in\mathbb R_+^p}\quad
    & \frac{\sigma_{\mathrm{port}}}{2}\bbeta^\top\bSigma\bbeta
      +\frac{1}{2\gamma_{\mathrm{port}}}\norm{\bbeta}_2^2
      -\bmu^\top\bbeta\\
\mathrm{s.t.}\quad
    & \vone^\top\bbeta\leq1,\qquad \norm{\bbeta}_0\leq k.
\end{aligned}
\label{eq:exp-portfolio}
\end{equation}
Here, $p$ is the number of assets, $\bbeta$ contains their nonnegative portfolio weights, $\bSigma$ is the return covariance matrix, and $\bmu$ contains the expected returns. The parameter $\sigma_{\mathrm{port}}$ scales the risk term, and $\gamma_{\mathrm{port}}$ controls ridge regularization. For the synthetic instances we set $\sigma_{\mathrm{port}}=1$ and $\gamma_{\mathrm{port}}=100/\sqrt{p}$. They use the budget and cardinality constraints shown above.

For the Yahoo Finance instances, we use a return-constrained variant. In this model the expected return is imposed as a minimum-return constraint and does not appear as a linear objective term:
\begin{equation}
\begin{aligned}
\min_{\bbeta\in\mathbb R_+^p}\quad
    & \frac{\sigma_{\mathrm{port}}}{2}\bbeta^\top\bSigma\bbeta
      +\frac{1}{2\gamma_{\mathrm{port}}}\norm{\bbeta}_2^2\\
\mathrm{s.t.}\quad
    & \vone^\top\bbeta\leq1,\qquad \bmu^\top\bbeta\geq t,\\
    & \norm{\bbeta}_0\leq k.
\end{aligned}
\label{eq:exp-portfolio-market}
\end{equation}
For these instances, $t>0$ is the data-specific return floor, set to $r_{\min}+0.3(r_{\max}-r_{\min})$ using the return band fixed for each benchmark instance. We set $\sigma_{\mathrm{port}}=1$ and $\gamma_{\mathrm{port}}=100/\sqrt{p}$. Thus, the synthetic and market-data results use distinct portfolio formulations, each matching its corresponding benchmark instances. In the market-data model, positivity and homogeneity of degree two force $\bmu^\top\bbeta=t$ at every feasible node optimum.

\subsection{Dataset Construction and Preprocessing}
\label{app:data-generation}
The synthetic BnB experiments use seeds $0,1,2$. Numerical inputs are fixed for the methods compared within each campaign; the standalone relaxation campaigns retain their recorded seed sets. We describe the construction and preprocessing for each problem class below.

\paragraph{Sparse linear and logistic regression.}
For the synthetic instances, we generate Gaussian designs with
\[
n=p\in\{1000,2000,4000,10000\},
\qquad
(\bSigma_{\bX})_{ij}=0.5^{|i-j|}.
\]
The generating coefficient vector $\bbeta^{\mathrm{true}}$ has ten unit entries at equally spaced positions and is zero elsewhere. We use this vector to generate linear responses with Gaussian noise of standard deviation $0.5$, or binary labels according to the logistic model.

For synthetic data, we generate the ten additional linear inequalities by
\[
C_{\ell j}\sim\mathcal N(0,1/p),
\qquad
b_{\mathrm{aff},\ell}=\bm{C}_{\ell,:}\bbeta^{\mathrm{true}}+|\omega_\ell|+0.5,
\qquad
\omega_\ell\sim\mathcal N(0,1),
\]
for $\ell\in[10]$ and $j\in[p]$, where $C_{\ell j}$ is the corresponding scalar entry of $\bm{C}$. The resulting slack at $\bbeta^{\mathrm{true}}$ is $|\omega_\ell|+0.5>0$, so the generating vector strictly satisfies these additional inequalities.

For the real-data experiments, we use Santander Value Prediction~\citep{santander} for linear regression and DOROTHEA~\citep{guyon2004result} for logistic regression. Their final dimensions $(n,p)$ are $(3557,4685)$ and $(1830,88666)$, respectively. We remove redundant features, balance DOROTHEA by sampling with replacement, and use the training portion of a fixed five-fold split. We center the features and scale them to unit norm using training statistics. We standardize the Santander responses without applying a logarithmic transformation. Ten reserved unit-norm rows define the inequalities
\[
\bc_\ell^\top\bbeta\leq0.5,\qquad \ell\in[10],
\]
where $\bc_\ell^\top$ is the corresponding row of $\bm{C}$. These rows are excluded from the fitting loss.

\paragraph{Separable quadratic uncapacitated facility location.}
We generate synthetic SQUFL instances with the library's seeded geometric generator, following \citet{gunluk2007minlp} and the standard quadratic facility-location structure represented in MINLPLib~\citep{bussieck2003minlplib}. Facility locations $\bx_i$ and customer locations $\by_j$ are sampled uniformly from $[0,1]^2$. We construct opening costs and allocation coefficients as
\[
c_i=\lceil U_i\rceil,\qquad U_i\sim\mathcal U(1,100),
\qquad
q_{ij}=50\norm{\bx_i-\by_j}_2.
\]
The result tables report the numbers of facilities and customers for each synthetic instance.

\paragraph{Sparse portfolio optimization.}
Following \citet{han2022twobytwo}, we construct dense synthetic covariance matrices from 20 random factors. We scale positive off-diagonal entries by $0.3$ and replace each diagonal entry with the sum of the absolute off-diagonal entries in its row plus independently sampled slack. Each slack is uniform on $[0,0.5\bar{s}]$, where $\bar{s}$ is the mean row sum of absolute off-diagonal entries before diagonal replacement. We sample the expected returns from
\[
\mu_i\sim\mathcal U\bigl(0.5\Sigma_{ii},\,1.5\Sigma_{ii}\bigr),
\qquad i\in[p],
\]
where $\Sigma_{ii}$ is the $i$th diagonal entry before normalization. We then jointly normalize the covariance matrix and expected returns so that the average asset variance is one. We reuse each generated instance for $k=5$ and $k=10$.

For the real-data experiments, we use the fixed Yahoo Finance datasets YF-27907 ($p=27{,}907$) and YF-35629 ($p=35{,}629$), each with $3039$ log-return observations; the reported portfolio BnB instances use $k=5$. We filter the prices and apply forward and backward filling. We then clip returns at the pooled $99.9$th percentile of absolute returns. Filling and clipping take place before the chronological split. We use these datasets for computational benchmarking.

We estimate expected returns and covariances from the training period. The covariance-estimation rule uses the sample covariance when the return history contains more observations than assets, and Ledoit--Wolf shrinkage otherwise~\citep{ledoit2004well}. For YF-27907 and YF-35629, we estimate the expected returns and Ledoit--Wolf covariances from the first $1519$ observations.

\paragraph{Asset sources, terms, and access.}
\label{app:asset-information}
DOROTHEA~\citep{guyon2004result} is distributed by \href{https://archive.ics.uci.edu/dataset/169/dorothea}{UCI} under \href{https://creativecommons.org/licenses/by/4.0/}{CC BY 4.0}.
Banco Santander's Value Prediction data~\citep{santander} are subject to \href{https://www.kaggle.com/competitions/santander-value-prediction-challenge/rules}{Kaggle competition rules}, which permit noncommercial academic use and restrict redistribution; users obtain them from the provider after accepting those rules.
Yahoo Finance market data remain subject to \href{https://legal.yahoo.com/us/en/yahoo/terms/otos/index.html}{Yahoo and data-provider terms}; no open redistribution license is asserted.
The anonymized supplement includes solver code, DOROTHEA/SANTANDER runners, synthetic generators, configurations, and input manifests under a submission-evaluation license; dependency licenses and dataset access information accompany it.
Fixed preprocessed real-data arrays are not bundled, and provider downloads alone do not reconstruct their recorded identities.
We use molecular descriptors, provider-anonymized Santander features, and public market series, without identity reconstruction or new participant-data collection; public release is not taken as evidence of individual consent.

\subsection{Computational Protocol}
\label{app:computational-protocol}

\paragraph{Hardware and software.}
CPU experiments use AMD EPYC processors, and GPU experiments use NVIDIA H100 accelerators. The CPU BnB campaign uses AMD EPYC 7713 processors with eight CPU threads per solve. The recorded software environment comprises Python 3.12.3, Gurobi 13.0.2, MOSEK 11.2.2, Clarabel 0.11.1, and SCS 3.2.11; our implementation uses PyTorch 2.11.0 with CUDA 12.8. GPU execution includes unbatched node solves and a batched variant that processes multiple active nodes together. The recorded GPU BnB configuration has a maximum batch size of 512; actual occupancy depends on the available active nodes. All computations, including the GPU runs, use double-precision arithmetic.
Here, ``safe'' denotes validity in exact arithmetic; rigorous floating-point certification is not claimed.

\paragraph{Stopping criteria and time budget.}
The target relative gap for standalone node relaxations and for node solves within BnB is $10^{-6}$. The target global BnB relative gap is $10^{-4}$. For our relaxation solver, given finite primal and dual bounds $P$ and $D$, we use
\[
\operatorname{gap}_{\mathrm{relax}}
=\frac{|P-D|}{\max\{10^{-10},|P|,|D|\}}.
\]
For the global BnB certificate, with incumbent value $U$ and global lower bound $L$, we use
\[
\operatorname{gap}_{\mathrm{BnB}}
=\frac{U-L}{\max\{10^{-10},|U|\}},\qquad L\leq U.
\]
The small denominator safeguard avoids division by zero. Gaps in the result tables are reported as percentages. All solvers receive the same requested global relative-gap tolerance. Each BnB run uses a 3600-second solver time limit. Data loading and model construction are timed separately where available; the reported BnB runtimes refer to the solver phase.

\paragraph{Branch-and-bound implementation.}
Our CPU and GPU trees use best-bound node selection; CPU and unbatched GPU runs process one node at a time, while the batched GPU streams up to 512. Children inherit the parent relaxation's primal and dual iterates. Regression branches on the free coordinate with $|\hat\beta_j|>10^{-12}$ maximizing the heuristic score $L_j\hat\beta_j^2/2-g_j\hat\beta_j$, where $\hat{\bbeta}$ is the node's stored primal reference, $g_j=(\bX^\top\nabla f(\bX\hat{\bbeta}))_j$, and $L_j=\rho\|\bX_{:,j}\|_2^2+2\lambda_2$. Here $\rho=1$ for squared loss and $1/4$ for logistic loss; if no free coordinate passes the nonzero test, all free coordinates are considered. SQUFL and portfolio select the most fractional free binary variable. Regression and portfolio node anchors project the root anchor onto the node. When a projected anchor fails the feasibility check, we solve the affine max-margin Phase-I problem by a first-order primal--dual method. SQUFL uses a closed-form node anchor when available and solves one-facility leaves exactly. A node anchor is reused for its relaxation; support-restricted solves construct and check a separate anchor. Incumbent generation uses a Phase-I method.

\paragraph{Scope of comparisons.}
Our BnB comparisons use Gurobi and MOSEK as general-purpose baselines; they do not include specialized methods for facility location~\citep{fischetti2016benders}, sparse regression and $k$-sparse GLMs~\citep{hazimeh2022sparse,liu2025scalable,liu2026gpu}, or mixed-integer quadratic optimization~\citep{stellato2018embedded}.

\paragraph{Repetitions and aggregation.}
The synthetic BnB tables report arithmetic means of runtimes, final gaps, and node counts over seeds $0,1,2$. In the synthetic repair ablation, no-repair stopping requires normalized primal violation at most $10^{-8}$ and raw relative objective gap at most $10^{-6}$ for two consecutive iterations; tree pruning uses the shared repaired dual bound. Iteration counts are pooled over processed nodes from seeds that converged within the time limit; time-limited seeds are excluded. Percentages express the iterations remaining relative to the no-repair baseline. The conjugate-evaluation microbenchmark follows the warm-repetition timing protocol stated in its caption.

\paragraph{Averaging and restarts.}
Our averaging and adaptive restart strategy follows the design of PDLP~\citep{applegate2021practical}; related acceleration methods include optimized Halpern iteration~\citep{park2022exact} and restarted Halpern PDHG~\citep{lu2407restarted}. We weight the running average of the iterates by their step sizes and evaluate the residual merit function for both the current iterate and this average. Restart tests are performed every 200 iterations after a minimum restart interval of 64 iterations. A restart is triggered when the smaller candidate residual falls below $0.2$ times its value at the preceding restart, or falls below $0.8$ times that value and subsequently increases, or when the current interval reaches $0.36$ times the total iteration count. We restart from the candidate with the smaller residual and adapt the step sizes and primal--dual balance. Repaired primal and dual bounds, rather than the restart residual, determine relaxation termination and node pruning. Theorem~\ref{theorem:convergence_rate} concerns a fixed certificate map and metric; it does not by itself establish convergence rates for these adaptive configurations.



\paragraph{Application variables and node splittings.}
The generic vector $\bbeta$ in Sections~3--4 denotes the entire decision vector. In the selector formulations above, this vector is $x=(\bbeta,\bz)$ (with the allocation matrix vectorized for SQUFL). For lifted regression, the loss matrix is $[\bX\ \mathbf{0}]$; constraint operators and the conjugate variable $u$ act on the full lifted space. When selectors are eliminated by partial minimization, the primal space instead consists of the coefficient or portfolio vector alone, and all operators and dual variables have that reduced dimension.
For integer branching in Section~\ref{subsec:convex-relaxation}, a fractional $c_j\in(l_j,u_j)$ gives children $[l_j,\lfloor c_j\rfloor]$ and $[\lceil c_j\rceil,u_j]$.

We distinguish the canonical splitting in the main text and Appendices~\ref{sec:base-algorithm}--\ref{app:dual-bounds} from the application splittings below. In the canonical splitting, the node box is block~0 of $h$. In an application splitting, domain restrictions and node fixings can instead be included in the proximable term $g_{\calN}$. Write
\[
 P_{\calN}(v)=f(A_{\calN}v)+g_{\calN}(v)+h_{\calN}(K_{\calN}v),\qquad
 h_{\calN}(q_1,\ldots,q_r)=\sum_{i=1}^r\delta_{D_{\calN,i}}(q_i),
\]
where $K_{\calN}$ stacks $r$ copies of the identity on the actual primal space and the sets $D_{\calN,i}$ contain the remaining constraints. Moving an indicator into $g_{\calN}$ leaves this objective unchanged pointwise. It changes the proximal splitting, however: certificates use $g_{\calN}^*$, $h_{\calN}^*$, and $A_{\calN}^T\zeta+u+K_{\calN}^T\nu$ for that splitting. The main-text certificate constructions apply with these substitutions; any residual-rate conclusion additionally requires Theorem~\ref{theorem:convergence_rate}'s assumptions for the actual map and metric. No equality of iterates between different splittings is asserted.

Let $Z_{\calN}=\{z\in[0,1]^d:z_j=0\ (j\in J_0),\ z_j=1\ (j\in J_1)\}$ encode the node's selector fixings, and let $Z_{\calN}^k=Z_{\calN}\cap\{\vone^Tz\leq k\}$. We use the closed perspective convention $a^2/0=0$ for $a=0$ and $+\infty$ otherwise. All reported results for our method use the perspective blocks below, including the unbounded perspective block for portfolios. Gurobi and MOSEK receive the corresponding perspective formulations, represented with rotated second-order-cone constraints where applicable.

\paragraph{Regression blocks.}
The perspective and ordinary big-$M$ blocks implemented for regression are, respectively,
\begin{align*}
 g_{\calN}^{\rm pers}(\bbeta)
 &=\inf_{\substack{z\in Z_{\calN}^k\\|\beta_j|\leq Mz_j}}
       \lambda_2\sum_j\frac{\beta_j^2}{z_j},\\
 g_{\calN}^{\rm bigM}(\bbeta)
 &=\lambda_2\norm{\bbeta}_2^2+
   \delta_{\{\bbeta:\exists z\in Z_{\calN}^k,\ |\beta_j|\leq Mz_j\}}(\bbeta).
\end{align*}
Here $A_{\calN}=\bX$, $f$ is the stated squared or logistic loss, and the remaining sets are $D_{\calN,i}=\{\bbeta:\bm C_{i,:}\bbeta\leq b_{{\rm aff},i}\}$. Each displayed infimum is exactly the partial minimization over selectors of its corresponding lifted node relaxation. The perspective block yields the bounded top-$k$ Huber formulation; the big-$M$ block is ridge plus the projected selector domain. They agree with Equation~\eqref{eq:exp-regression} at binary selectors, but the perspective relaxation can be stronger than merely replacing $z\in\{0,1\}^p$ by $z\in[0,1]^p$.

\paragraph{Facility-location blocks.}
With $v=(\operatorname{vec}\bbeta,z)$, take $A_{\calN}=I$, $f=0$, and
\[
 g_{\calN}^{\rm pers}(v)=\sum_i c_i z_i+
 \sum_{i,j}q_{ij}\frac{\beta_{ij}^2}{z_i}
 +\delta_{\{z\in Z_{\calN},\ 0\leq\beta_{ij}\leq z_i\}}(v).
\]
The ordinary quadratic variant replaces $\beta_{ij}^2/z_i$ by $\beta_{ij}^2$. The remaining sets are the customer-covering halfspaces $D_{\calN,j}=\{v:\sum_i\beta_{ij}\geq1\}$. These $n$ halfspaces act on disjoint allocation coordinates and are implemented as one block with a separable projection, so $K_{\calN}$ has a single identity copy for this block. This is a grouping of the lifted node objective and domain, so it changes neither that relaxation nor its optimum. The perspective and ordinary variants coincide for binary $z$, but generally differ for fractional $z$. The preceding covering argument applies to both, since reducing nonnegative allocations cannot increase either quadratic cost.

\paragraph{Portfolio blocks.}
For the perspective portfolio relaxation, $A_{\calN}=I$ and
\[
 f(\bbeta)=\frac{\sigma_{\rm port}}2\bbeta^T\bSigma\bbeta-r^T\bbeta,
 \qquad
 g_{\calN}(\bbeta)=\inf_{\substack{z\in Z_{\calN}^k\\\bbeta\geq0}}
       \frac1{2\gamma_{\rm port}}\sum_j\frac{\beta_j^2}{z_j},
\]
where $r=\bmu$ for synthetic instances and $r=0$ for the market-data instances. The remaining sets impose the budget and, for market data, the minimum return. Partial minimization over $z$ gives exactly the one-sided squared $k$-support block of this lifted perspective relaxation. At binary selectors it reproduces the stated sparse model. The bounded portfolio variant additionally imposes $\beta_j\leq Mz_j$ inside the infimum; this is a different continuous relaxation and is equivalent to the intended integer model only when $M$ is a valid weight bound.

The bounded regression and facility domains give globally Lipschitz conjugates. The unbounded portfolio block has a finite conjugate, but not a globally Lipschitz one; the repair-rate conclusion requiring that hypothesis is not asserted for it. Finite absorbing certificates remain valid. The budget-constrained nonnegative portfolio feasible set is compact, permitting the support-correction construction under its stated assumptions.

\paragraph{Anchor failure and infeasibility.}
Node anchors are checked against the node restrictions. In the repaired regression and portfolio paths, failure to obtain an anchor retains the inherited lower bound; it is not used as an infeasibility certificate. For SQUFL, a node with no admissible facility is structurally infeasible, while a node with one admissible facility has an explicit fixed-support solution. Other anchor failures provide no new finite lower certificate. These mechanisms do not constitute a general infeasibility oracle for arbitrary convex constraints. An unresolved feasibility search must not be reported as certified infeasibility.
