# Supplementary material for: First-Order Primal-Dual Repairs for Scalable Branch and Bound
Source: arXiv:2610.26509 source file (2026-10-19)
Supplement: Supplementary file 10 [file H_experiments.tex]

\clearpage
\section{Additional Experimental Results}
\label{app:additional-experiments}

This appendix reports node-relaxation times (Table~\ref{tab:all-relaxations}), BnB results (Tables~\ref{tab:okglm-bnb-wide-1e-6}--\ref{tab:synthetic-bnb-global-1e-6}), sample SDs (Tables~\ref{tab:synthetic-bnb-sd-1e-4}--\ref{tab:synthetic-bnb-sd-1e-6}), repair ablations (Table~\ref{tab:synthetic-repair-ablation}), component times (Table~\ref{tab:bnb-component-times}), and dual-certificate trajectories (Figures~\ref{fig:synthetic-dual-linear}--\ref{fig:synthetic-dual-portfolio}). The tolerance campaigns are separate except for reused regression runs identified in Table~\ref{tab:synthetic-bnb-global-1e-6}. For repair ablation, each instance and seed uses one best-bound tree with a fixed incumbent certified to relative gap $10^{-4}$. The four stopping counts share each node trajectory; pruning uses a repaired dual bound. Means pool nodes from completed trees.
Tables~\ref{table:repair_ablation} and~\ref{tab:synthetic-repair-ablation} report best-case iteration savings with a fixed, pre-certified incumbent on shared trajectories, rather than end-to-end BnB speedups.

In Table~\ref{tab:okglm-bnb-wide}, completed CPU comparisons give speedups of $16$--$84\times$ over Gurobi and MOSEK; SANTANDER and both YF instances reach the target only in our GPU configurations.
On synthetic portfolios, Gurobi is fastest or tied at $p\leq2000$; our batched GPU solver is $2.3\times$ and $24\times$ faster than Gurobi at $p=4000$ and $p=10000$, respectively (Table~\ref{tab:synthetic-bnb-global-1e-4}). At $p=10000$, Gurobi reaches the time limit at global gap tolerance $10^{-6}$ (Table~\ref{tab:synthetic-bnb-global-1e-6}).

\begin{table*}[!htbp]
\centering
\setlength{\abovecaptionskip}{0pt}
\setlength{\belowcaptionskip}{6pt}
\caption{Single-node relaxation times (s) at relative gap $10^{-6}$; synthetic CPU results correspond to Figure~\ref{fig:noderelaxations}.}
\label{tab:all-relaxations}
\label{tab:okglm-linear-relax}
\label{tab:okglm-logistic-relax}
\label{tab:squfl-relax}
\label{tab:portfolio-relax}
\small
\setlength{\tabcolsep}{3pt}
\renewcommand{\arraystretch}{1.12}
\begin{tabular*}{\linewidth}{@{\extracolsep{\fill}}lrrrrrrr@{}}
\toprule
Instance & Gurobi & MOSEK & Clarabel & SCS & Ours-Traditional & Ours CPU & Ours GPU \\
\midrule
\multicolumn{8}{@{}l}{\emph{Linear regression}} \\
$n=p=1000$ & 12.1 & 1.7 & 25.4 & 507.9 & 1.99 & \textbf{0.98} & 1.6 \\
$n=p=2000$ & 93.7 & 7.6 & 151.4 & 1536.6 & 6.03 & 2.65 & \textbf{1.3} \\
$n=p=4000$ & 768.8 & 40.8 & TL & TL & 17.53 & 6.68 & \textbf{1.0} \\
$n=p=10000$ & TL & 489.4 & TL & TL & 81.51 & 27.27 & \textbf{1.3} \\
SANTANDER & TL & 269.9 & TL & TL & 4.9 & 4.9 & \textbf{0.7} \\
\midrule
\multicolumn{8}{@{}l}{\emph{Logistic regression}} \\
$n=p=1000$ & TL & 4.6 & 18.1 & 696.7 & 1.77 & \textbf{0.27} & 1.4 \\
$n=p=2000$ & TL & 27.6 & 33.2 & TL & 5.04 & \textbf{0.67} & 0.7 \\
$n=p=4000$ & TL & 199.6 & 199.7 & TL & 17.61 & 2.04 & \textbf{0.7} \\
$n=p=10000$ & TL & 2905.7 & TL & TL & 107.99 & 11.63 & \textbf{0.8} \\
DOROTHEA & TL & 769.5 & TL & TL & 112.3 & 88.5 & \textbf{5.7} \\
\midrule
\multicolumn{8}{@{}l}{\emph{SQUFL}} \\
$m=150$, $n=750$ & 28.6 & 12.9 & 15.0 & 1963.9 & \textbf{0.292} & 0.33 & 0.7 \\
$m=200$, $n=1000$ & 51.5 & 24.3 & 29.4 & TL & \textbf{0.538} & 0.62 & 0.6 \\
$m=500$, $n=2500$ & 567.3 & 188.4 & 342.5 & TL & 5.751 & 4.14 & \textbf{0.7} \\
\midrule
\multicolumn{8}{@{}l}{\emph{Portfolio: synthetic ($k=5$)}} \\
$p=2000$ & 25.6 & 12.7 & 6.56 & 10.6 & 1.38 & \textbf{1.25} & 2.52 \\
$p=4000$ & 317.5 & 72.8 & 39.0 & 159.0 & 10.65 & 10.58 & \textbf{3.69} \\
$p=10000$ & TL & 755.1 & 178.8 & 1300.1 & 44.54 & 40.62 & \textbf{9.45} \\
$p=12000$ & TL & 1245.4 & 236.4 & 1826.8 & 60.85 & 56.25 & \textbf{5.24} \\
\midrule
\multicolumn{8}{@{}l}{\emph{Portfolio: market data}} \\
YF-35629 & 2013.1 & 385.7 & 3115.7 & TL & 1480.1 & 1600.8 & \textbf{64.2} \\
YF-27907 & TL & TL & 2123.4 & TL & 3269.2 & 2376.2 & \textbf{198.4} \\
\bottomrule
\end{tabular*}

\end{table*}

\clearpage
\input{sections/Appendix/FOUR_BNB_APPENDIX_TABLES}

\clearpage
\begin{table*}[!htbp]
\centering
\setlength{\abovecaptionskip}{0pt}
\setlength{\belowcaptionskip}{6pt}
\caption{Repair ablation on synthetic instances at global relative gap tolerance of $10^{-4}$. Parentheses give the percentage of iterations remaining relative to no repair, $100\,I/I_{\mathrm{raw}}$, computed from the displayed means. Bold marks the lowest iteration count in each row.}
\label{tab:synthetic-repair-ablation}
\small
\setlength{\tabcolsep}{2.7pt}
\renewcommand{\arraystretch}{1.15}
\begin{tabular*}{\linewidth}{@{\extracolsep{\fill}}lrrrr@{}}
\toprule
Instance & No repair & Primal & Dual & Primal+dual \\
\midrule
\multicolumn{5}{@{}l}{\emph{Linear regression}} \\
$n=p=1000$ & 163.2 & 56.5\,(35\%) & 111.1\,(68\%) & \textbf{4.4}\,(3\%) \\
$n=p=2000$ & 109.3 & 38.6\,(35\%) & 74.1\,(68\%) & \textbf{3.5}\,(3\%) \\
$n=p=4000$ & 71.8 & 29.3\,(41\%) & 45.4\,(63\%) & \textbf{2.9}\,(4\%) \\
$n=p=10000$ & 47.8 & 21.5\,(45\%) & 28.9\,(60\%) & \textbf{2.6}\,(5\%) \\
\midrule
\multicolumn{5}{@{}l}{\emph{Logistic regression}} \\
$n=p=1000$ & 35.6 & 17.6\,(49\%) & 20.3\,(57\%) & \textbf{2.2}\,(6\%) \\
$n=p=2000$ & 39.9 & 19.6\,(49\%) & 23.1\,(58\%) & \textbf{2.9}\,(7\%) \\
$n=p=4000$ & 34.2 & 17.3\,(51\%) & 19.7\,(58\%) & \textbf{2.8}\,(8\%) \\
$n=p=10000$ & 31.2 & 16.2\,(52\%) & 18.0\,(58\%) & \textbf{3.0}\,(10\%) \\
\midrule
\multicolumn{5}{@{}l}{\emph{SQUFL}} \\
$m=150,\ n=750$ & 68.7 & 51.8\,(75\%) & 48.7\,(71\%) & \textbf{31.8}\,(46\%) \\
$m=200,\ n=1000$ & 64.1 & 50.3\,(78\%) & 39.8\,(62\%) & \textbf{26.0}\,(41\%) \\
$m=500,\ n=2500$ & 86.0 & 64.4\,(75\%) & 51.0\,(59\%) & \textbf{29.3}\,(34\%) \\
\midrule
\multicolumn{5}{@{}l}{\emph{Portfolio (k = 5)}} \\
$p=1000$ & 3111.4 & 2019.4\,(65\%) & 1667.1\,(54\%) & \textbf{575.1}\,(18\%) \\
$p=2000$ & 7645.5 & 5074.8\,(66\%) & 3872.4\,(51\%) & \textbf{1301.7}\,(17\%) \\
$p=4000$ & 16861.5 & 11579.6\,(69\%) & 8845.2\,(52\%) & \textbf{3563.3}\,(21\%) \\
$p=10000$ & 53650.0 & 38392.4\,(72\%) & 30158.0\,(56\%) & \textbf{14900.4}\,(28\%) \\
\bottomrule
\end{tabular*}

\end{table*}


\clearpage
\subsection{Component timings}
\label{app:bnb-component-times}
Table~\ref{tab:bnb-component-times} uses the batched runs of Tables~\ref{tab:okglm-bnb-wide} and~\ref{tab:synthetic-bnb-global-1e-4}: three-seed means for synthetic instances and single runs for real instances. Times are host-observed totals per run. Other is total solver time minus the three phase totals, before rounding; incumbent recovery includes the work to find a feasible point on the selected support and the subsequent restricted-support re-solve.
\input{sections/Appendix/bnb_component_times}

\subsection{Dual-certificate trajectories on synthetic relaxations}
\label{app:synthetic-dual-trajectories}
We plot $P_{\calN}^t$, $\mathrm{LB}_{\mathrm{repair}}^t$, and $\mathrm{LB}_{\mathrm{violation}}^t$ along the same root-relaxation trajectory; $\mathrm{LB}_{\mathrm{violation}}^t$ includes the support correction $\sigma_D$. Each row fixes an instance size; columns show seeds 0, 1, and 2 from left to right. The y-axis is the relative objective deviation from the midpoint of the terminal certified interval; vertical limits are shared within each row. The x-axis counts iterations.

\begin{figure*}[!p]
\centering
\begin{minipage}{0.325\linewidth}
\centering\small Seed 0
\end{minipage}\hfill
\begin{minipage}{0.325\linewidth}
\centering\small Seed 1
\end{minipage}\hfill
\begin{minipage}{0.325\linewidth}
\centering\small Seed 2
\end{minipage}
\par\smallskip
\begin{minipage}{0.325\linewidth}
\centering\includegraphics[width=\linewidth]{figures/dual_certificate_ablation/linear/000_okglm_linear_p1000_s0.pdf}
\end{minipage}\hfill
\begin{minipage}{0.325\linewidth}
\centering\includegraphics[width=\linewidth]{figures/dual_certificate_ablation/linear/001_okglm_linear_p1000_s1.pdf}
\end{minipage}\hfill
\begin{minipage}{0.325\linewidth}
\centering\includegraphics[width=\linewidth]{figures/dual_certificate_ablation/linear/002_okglm_linear_p1000_s2.pdf}
\end{minipage}
\par\smallskip
\begin{minipage}{0.325\linewidth}
\centering\includegraphics[width=\linewidth]{figures/dual_certificate_ablation/linear/003_okglm_linear_p2000_s0.pdf}
\end{minipage}\hfill
\begin{minipage}{0.325\linewidth}
\centering\includegraphics[width=\linewidth]{figures/dual_certificate_ablation/linear/004_okglm_linear_p2000_s1.pdf}
\end{minipage}\hfill
\begin{minipage}{0.325\linewidth}
\centering\includegraphics[width=\linewidth]{figures/dual_certificate_ablation/linear/005_okglm_linear_p2000_s2.pdf}
\end{minipage}
\par\smallskip
\begin{minipage}{0.325\linewidth}
\centering\includegraphics[width=\linewidth]{figures/dual_certificate_ablation/linear/006_okglm_linear_p4000_s0.pdf}
\end{minipage}\hfill
\begin{minipage}{0.325\linewidth}
\centering\includegraphics[width=\linewidth]{figures/dual_certificate_ablation/linear/007_okglm_linear_p4000_s1.pdf}
\end{minipage}\hfill
\begin{minipage}{0.325\linewidth}
\centering\includegraphics[width=\linewidth]{figures/dual_certificate_ablation/linear/008_okglm_linear_p4000_s2.pdf}
\end{minipage}
\par\smallskip
\begin{minipage}{0.325\linewidth}
\centering\includegraphics[width=\linewidth]{figures/dual_certificate_ablation/linear/009_okglm_linear_p10000_s0.pdf}
\end{minipage}\hfill
\begin{minipage}{0.325\linewidth}
\centering\includegraphics[width=\linewidth]{figures/dual_certificate_ablation/linear/010_okglm_linear_p10000_s1.pdf}
\end{minipage}\hfill
\begin{minipage}{0.325\linewidth}
\centering\includegraphics[width=\linewidth]{figures/dual_certificate_ablation/linear/011_okglm_linear_p10000_s2.pdf}
\end{minipage}
\caption{Linear regression synthetic root relaxations. Rows show the instance sizes in increasing order; columns are seeds 0, 1, and 2. Points show $P_{\calN}^t$, $\mathrm{LB}_{\mathrm{repair}}^t$, and $\mathrm{LB}_{\mathrm{violation}}^t$ at every iteration.}
\label{fig:synthetic-dual-linear}
\end{figure*}

\clearpage

\begin{figure*}[!p]
\centering
\begin{minipage}{0.325\linewidth}
\centering\small Seed 0
\end{minipage}\hfill
\begin{minipage}{0.325\linewidth}
\centering\small Seed 1
\end{minipage}\hfill
\begin{minipage}{0.325\linewidth}
\centering\small Seed 2
\end{minipage}
\par\smallskip
\begin{minipage}{0.325\linewidth}
\centering\includegraphics[width=\linewidth]{figures/dual_certificate_ablation/logistic/012_okglm_logistic_p1000_s0.pdf}
\end{minipage}\hfill
\begin{minipage}{0.325\linewidth}
\centering\includegraphics[width=\linewidth]{figures/dual_certificate_ablation/logistic/013_okglm_logistic_p1000_s1.pdf}
\end{minipage}\hfill
\begin{minipage}{0.325\linewidth}
\centering\includegraphics[width=\linewidth]{figures/dual_certificate_ablation/logistic/014_okglm_logistic_p1000_s2.pdf}
\end{minipage}
\par\smallskip
\begin{minipage}{0.325\linewidth}
\centering\includegraphics[width=\linewidth]{figures/dual_certificate_ablation/logistic/015_okglm_logistic_p2000_s0.pdf}
\end{minipage}\hfill
\begin{minipage}{0.325\linewidth}
\centering\includegraphics[width=\linewidth]{figures/dual_certificate_ablation/logistic/016_okglm_logistic_p2000_s1.pdf}
\end{minipage}\hfill
\begin{minipage}{0.325\linewidth}
\centering\includegraphics[width=\linewidth]{figures/dual_certificate_ablation/logistic/017_okglm_logistic_p2000_s2.pdf}
\end{minipage}
\par\smallskip
\begin{minipage}{0.325\linewidth}
\centering\includegraphics[width=\linewidth]{figures/dual_certificate_ablation/logistic/018_okglm_logistic_p4000_s0.pdf}
\end{minipage}\hfill
\begin{minipage}{0.325\linewidth}
\centering\includegraphics[width=\linewidth]{figures/dual_certificate_ablation/logistic/019_okglm_logistic_p4000_s1.pdf}
\end{minipage}\hfill
\begin{minipage}{0.325\linewidth}
\centering\includegraphics[width=\linewidth]{figures/dual_certificate_ablation/logistic/020_okglm_logistic_p4000_s2.pdf}
\end{minipage}
\par\smallskip
\begin{minipage}{0.325\linewidth}
\centering\includegraphics[width=\linewidth]{figures/dual_certificate_ablation/logistic/021_okglm_logistic_p10000_s0.pdf}
\end{minipage}\hfill
\begin{minipage}{0.325\linewidth}
\centering\includegraphics[width=\linewidth]{figures/dual_certificate_ablation/logistic/022_okglm_logistic_p10000_s1.pdf}
\end{minipage}\hfill
\begin{minipage}{0.325\linewidth}
\centering\includegraphics[width=\linewidth]{figures/dual_certificate_ablation/logistic/023_okglm_logistic_p10000_s2.pdf}
\end{minipage}
\caption{Logistic regression synthetic root relaxations. Rows show the instance sizes in increasing order; columns are seeds 0, 1, and 2. Points show $P_{\calN}^t$, $\mathrm{LB}_{\mathrm{repair}}^t$, and $\mathrm{LB}_{\mathrm{violation}}^t$ at every iteration.}
\label{fig:synthetic-dual-logistic}
\end{figure*}

\clearpage

\begin{figure*}[!p]
\centering
\begin{minipage}{0.325\linewidth}
\centering\small Seed 0
\end{minipage}\hfill
\begin{minipage}{0.325\linewidth}
\centering\small Seed 1
\end{minipage}\hfill
\begin{minipage}{0.325\linewidth}
\centering\small Seed 2
\end{minipage}
\par\smallskip
\begin{minipage}{0.325\linewidth}
\centering\includegraphics[width=\linewidth]{figures/dual_certificate_ablation/squfl/036_squfl_m150_n750_s0.pdf}
\end{minipage}\hfill
\begin{minipage}{0.325\linewidth}
\centering\includegraphics[width=\linewidth]{figures/dual_certificate_ablation/squfl/037_squfl_m150_n750_s1.pdf}
\end{minipage}\hfill
\begin{minipage}{0.325\linewidth}
\centering\includegraphics[width=\linewidth]{figures/dual_certificate_ablation/squfl/038_squfl_m150_n750_s2.pdf}
\end{minipage}
\par\smallskip
\begin{minipage}{0.325\linewidth}
\centering\includegraphics[width=\linewidth]{figures/dual_certificate_ablation/squfl/039_squfl_m200_n1000_s0.pdf}
\end{minipage}\hfill
\begin{minipage}{0.325\linewidth}
\centering\includegraphics[width=\linewidth]{figures/dual_certificate_ablation/squfl/040_squfl_m200_n1000_s1.pdf}
\end{minipage}\hfill
\begin{minipage}{0.325\linewidth}
\centering\includegraphics[width=\linewidth]{figures/dual_certificate_ablation/squfl/041_squfl_m200_n1000_s2.pdf}
\end{minipage}
\par\smallskip
\begin{minipage}{0.325\linewidth}
\centering\includegraphics[width=\linewidth]{figures/dual_certificate_ablation/squfl/042_squfl_m500_n2500_s0.pdf}
\end{minipage}\hfill
\begin{minipage}{0.325\linewidth}
\centering\includegraphics[width=\linewidth]{figures/dual_certificate_ablation/squfl/043_squfl_m500_n2500_s1.pdf}
\end{minipage}\hfill
\begin{minipage}{0.325\linewidth}
\centering\includegraphics[width=\linewidth]{figures/dual_certificate_ablation/squfl/044_squfl_m500_n2500_s2.pdf}
\end{minipage}
\caption{SQUFL synthetic root relaxations. Rows show the instance sizes in increasing order; columns are seeds 0, 1, and 2. Points show $P_{\calN}^t$, $\mathrm{LB}_{\mathrm{repair}}^t$, and $\mathrm{LB}_{\mathrm{violation}}^t$ every 50 iterations (including the first and last).}
\label{fig:synthetic-dual-squfl}
\end{figure*}

\clearpage

\begin{figure*}[!p]
\centering
\begin{minipage}{0.325\linewidth}
\centering\small Seed 0
\end{minipage}\hfill
\begin{minipage}{0.325\linewidth}
\centering\small Seed 1
\end{minipage}\hfill
\begin{minipage}{0.325\linewidth}
\centering\small Seed 2
\end{minipage}
\par\smallskip
\begin{minipage}{0.325\linewidth}
\centering\includegraphics[width=\linewidth]{figures/dual_certificate_ablation/portfolio/045_portfolio_p1000_s0.pdf}
\end{minipage}\hfill
\begin{minipage}{0.325\linewidth}
\centering\includegraphics[width=\linewidth]{figures/dual_certificate_ablation/portfolio/046_portfolio_p1000_s1.pdf}
\end{minipage}\hfill
\begin{minipage}{0.325\linewidth}
\centering\includegraphics[width=\linewidth]{figures/dual_certificate_ablation/portfolio/047_portfolio_p1000_s2.pdf}
\end{minipage}
\par\smallskip
\begin{minipage}{0.325\linewidth}
\centering\includegraphics[width=\linewidth]{figures/dual_certificate_ablation/portfolio/024_portfolio_p2000_s0.pdf}
\end{minipage}\hfill
\begin{minipage}{0.325\linewidth}
\centering\includegraphics[width=\linewidth]{figures/dual_certificate_ablation/portfolio/025_portfolio_p2000_s1.pdf}
\end{minipage}\hfill
\begin{minipage}{0.325\linewidth}
\centering\includegraphics[width=\linewidth]{figures/dual_certificate_ablation/portfolio/026_portfolio_p2000_s2.pdf}
\end{minipage}
\par\smallskip
\begin{minipage}{0.325\linewidth}
\centering\includegraphics[width=\linewidth]{figures/dual_certificate_ablation/portfolio/027_portfolio_p4000_s0.pdf}
\end{minipage}\hfill
\begin{minipage}{0.325\linewidth}
\centering\includegraphics[width=\linewidth]{figures/dual_certificate_ablation/portfolio/028_portfolio_p4000_s1.pdf}
\end{minipage}\hfill
\begin{minipage}{0.325\linewidth}
\centering\includegraphics[width=\linewidth]{figures/dual_certificate_ablation/portfolio/029_portfolio_p4000_s2.pdf}
\end{minipage}
\par\smallskip
\begin{minipage}{0.325\linewidth}
\centering\includegraphics[width=\linewidth]{figures/dual_certificate_ablation/portfolio/030_portfolio_p10000_s0.pdf}
\end{minipage}\hfill
\begin{minipage}{0.325\linewidth}
\centering\includegraphics[width=\linewidth]{figures/dual_certificate_ablation/portfolio/031_portfolio_p10000_s1.pdf}
\end{minipage}\hfill
\begin{minipage}{0.325\linewidth}
\centering\includegraphics[width=\linewidth]{figures/dual_certificate_ablation/portfolio/032_portfolio_p10000_s2.pdf}
\end{minipage}
\caption{Portfolio synthetic root relaxations. Rows show the instance sizes in increasing order; columns are seeds 0, 1, and 2. Points show $P_{\calN}^t$, $\mathrm{LB}_{\mathrm{repair}}^t$, and $\mathrm{LB}_{\mathrm{violation}}^t$ every 10 iterations (including the first and last).}
\label{fig:synthetic-dual-portfolio}
\end{figure*}
