# Supplementary material for: First-Order Primal-Dual Repairs for Scalable Branch and Bound
Source: arXiv:2610.26509 source file (2026-10-19)
Supplement: Supplementary file 11 [file bnb_component_times.tex]

\begin{table*}[!htbp]
\centering
\caption{Batched BnB phase totals (s) at global relative gap $10^{-4}$.}
\label{tab:bnb-component-times}
\small
\setlength{\tabcolsep}{5pt}
\renewcommand{\arraystretch}{1.12}
\begin{tabular*}{\linewidth}{@{\extracolsep{\fill}}lrrrrr@{}}
\toprule
Instance & Node anchor & Lower bounds & Incumbent & Other & Total \\
\midrule
\multicolumn{6}{@{}l}{\emph{Linear regression}} \\
$n=p=1000$ & 0.08 & 2.99 & 0.09 & 0.03 & 3.18 \\
$n=p=2000$ & 0.06 & 1.62 & 0.09 & 0.03 & 1.79 \\
$n=p=4000$ & 0.06 & 1.14 & 0.09 & 0.03 & 1.31 \\
$n=p=10000$ & 0.06 & 1.33 & 0.09 & 0.03 & 1.51 \\
SANTANDER & 0.90 & 18.42 & 51.86 & 3.04 & 74.23 \\
\midrule
\multicolumn{6}{@{}l}{\emph{Logistic regression }} \\
$n=p=1000$ & 0.75 & 2.07 & 3.67 & 2.09 & 8.57 \\
$n=p=2000$ & 0.13 & 0.75 & 0.45 & 0.24 & 1.56 \\
$n=p=4000$ & 0.08 & 0.67 & 0.27 & 0.11 & 1.13 \\
$n=p=10000$ & 0.07 & 0.82 & 0.19 & 0.06 & 1.15 \\
DOROTHEA & 0.07 & 4.94 & 0.69 & 0.06 & 5.75 \\
\midrule
\multicolumn{6}{@{}l}{\emph{SQUFL}} \\
$m=150,\ n=750$ & 0.03 & 0.98 & 1.07 & 0.02 & 2.11 \\
$m=200,\ n=1000$ & 0.04 & 0.66 & 0.55 & 0.01 & 1.26 \\
$m=500,\ n=2500$ & 0.04 & 0.82 & 0.63 & 0.01 & 1.50 \\
\midrule
\multicolumn{6}{@{}l}{\emph{Portfolio: synthetic}} \\
$p=1000$ & 0.05 & 11.39 & 6.96 & 0.22 & 18.62 \\
$p=2000$ & 0.07 & 11.35 & 6.44 & 0.18 & 18.04 \\
$p=4000$ & 0.06 & 15.52 & 11.54 & 0.33 & 27.44 \\
$p=10000$ & 0.09 & 26.44 & 22.77 & 0.80 & 50.11 \\
\midrule
\multicolumn{6}{@{}l}{\emph{Portfolio: market data}} \\
YF-35629 & 7.65 & 187.44 & 47.57 & 5.59 & 248.26 \\
YF-27907 & 4.03 & 126.08 & 38.11 & 7.34 & 175.56 \\
\bottomrule
\end{tabular*}
\end{table*}
